# Supplementary material for: Spectral variations among different scenarios of PAH processing or formation
Source: arXiv:2302.03678 source file (2023-02-07)

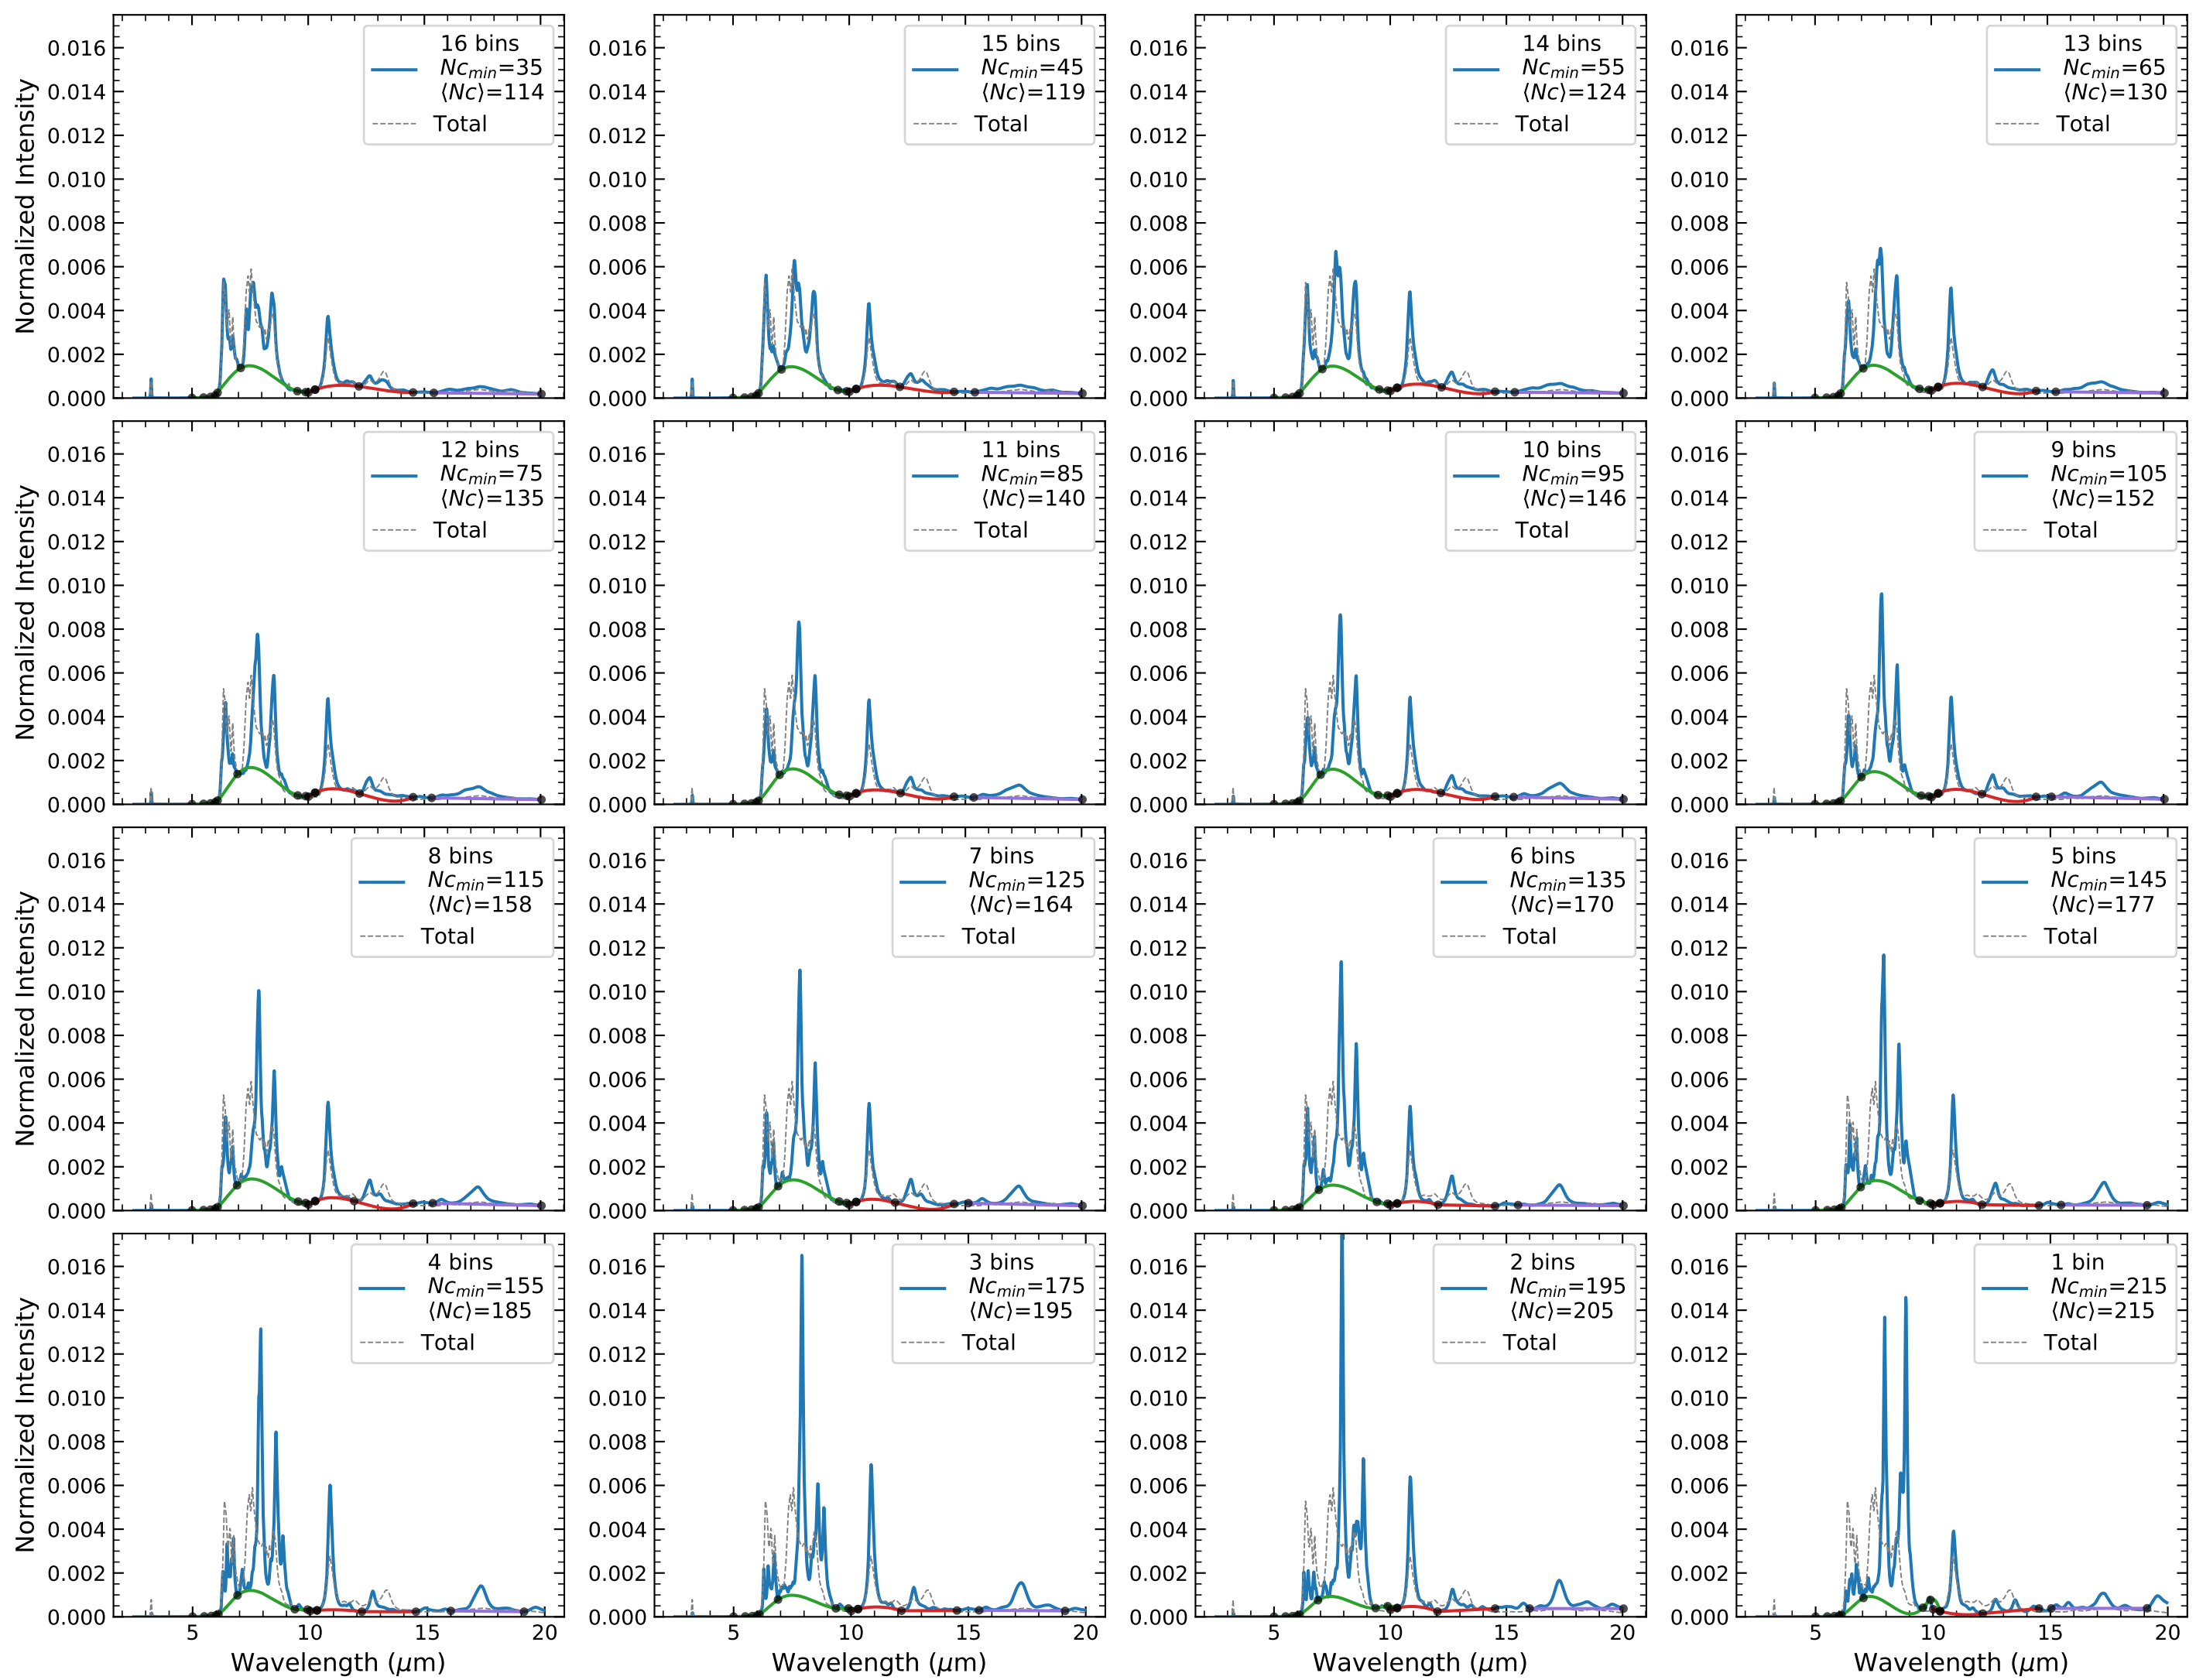

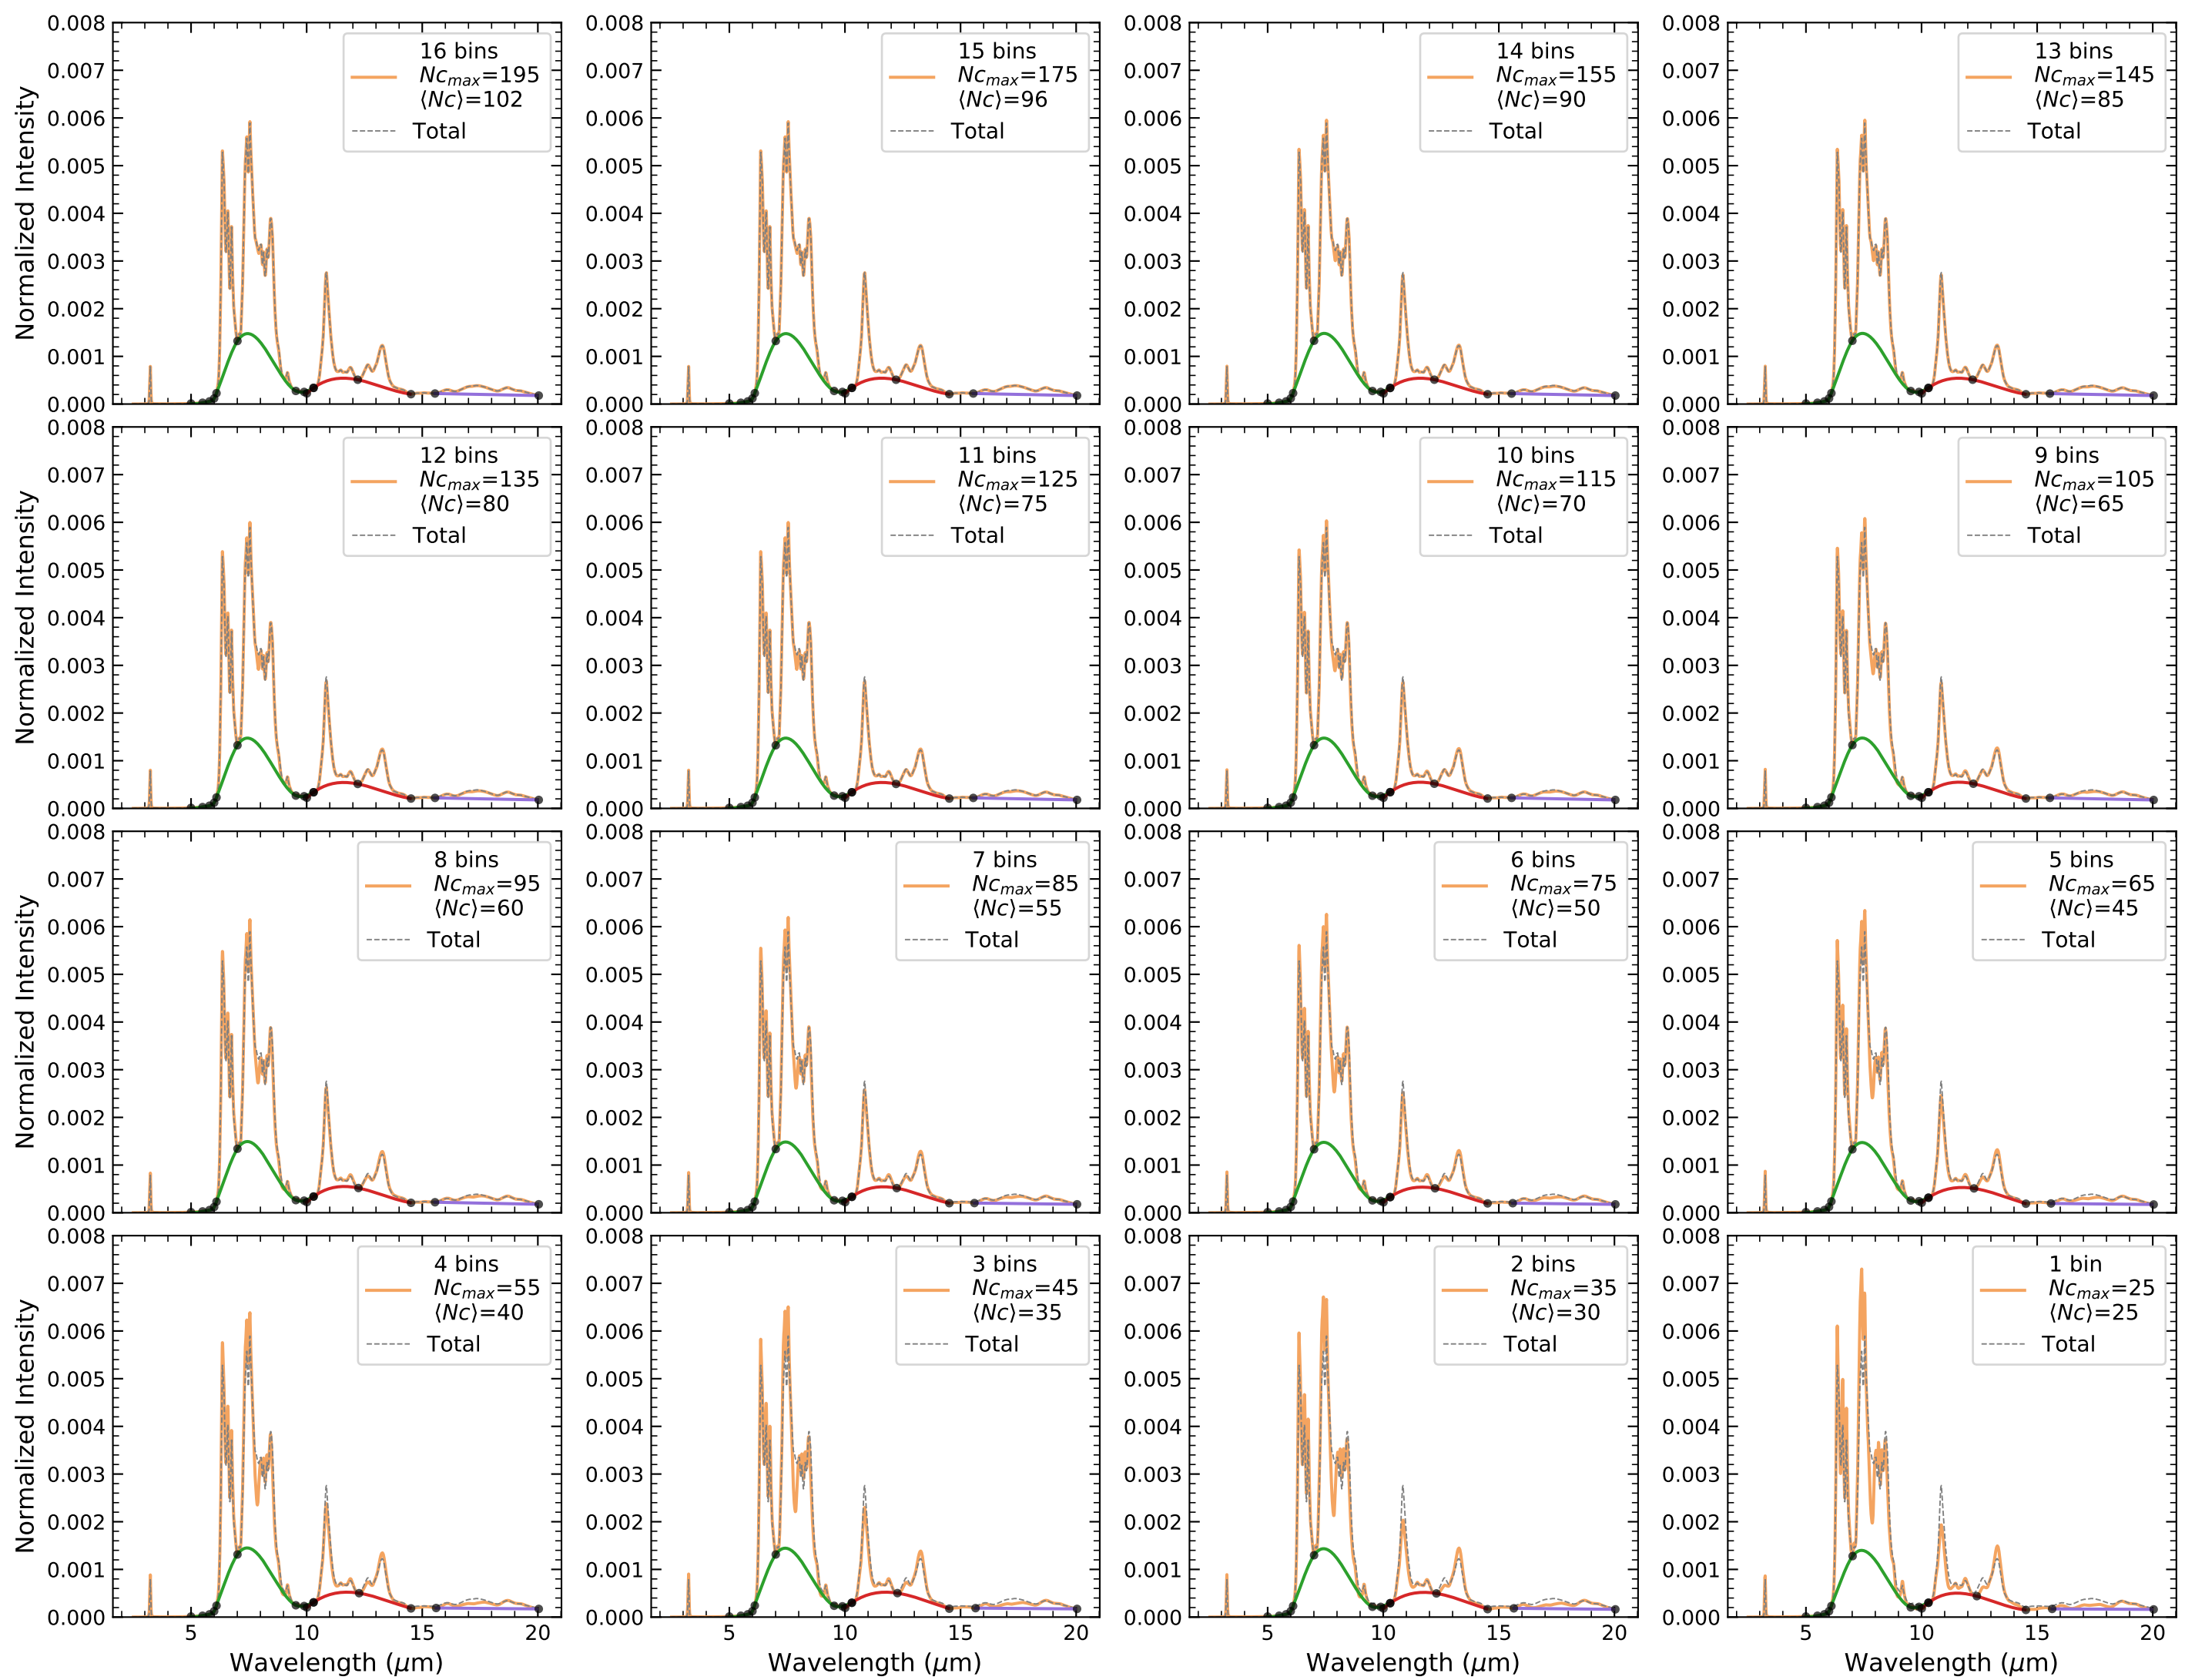

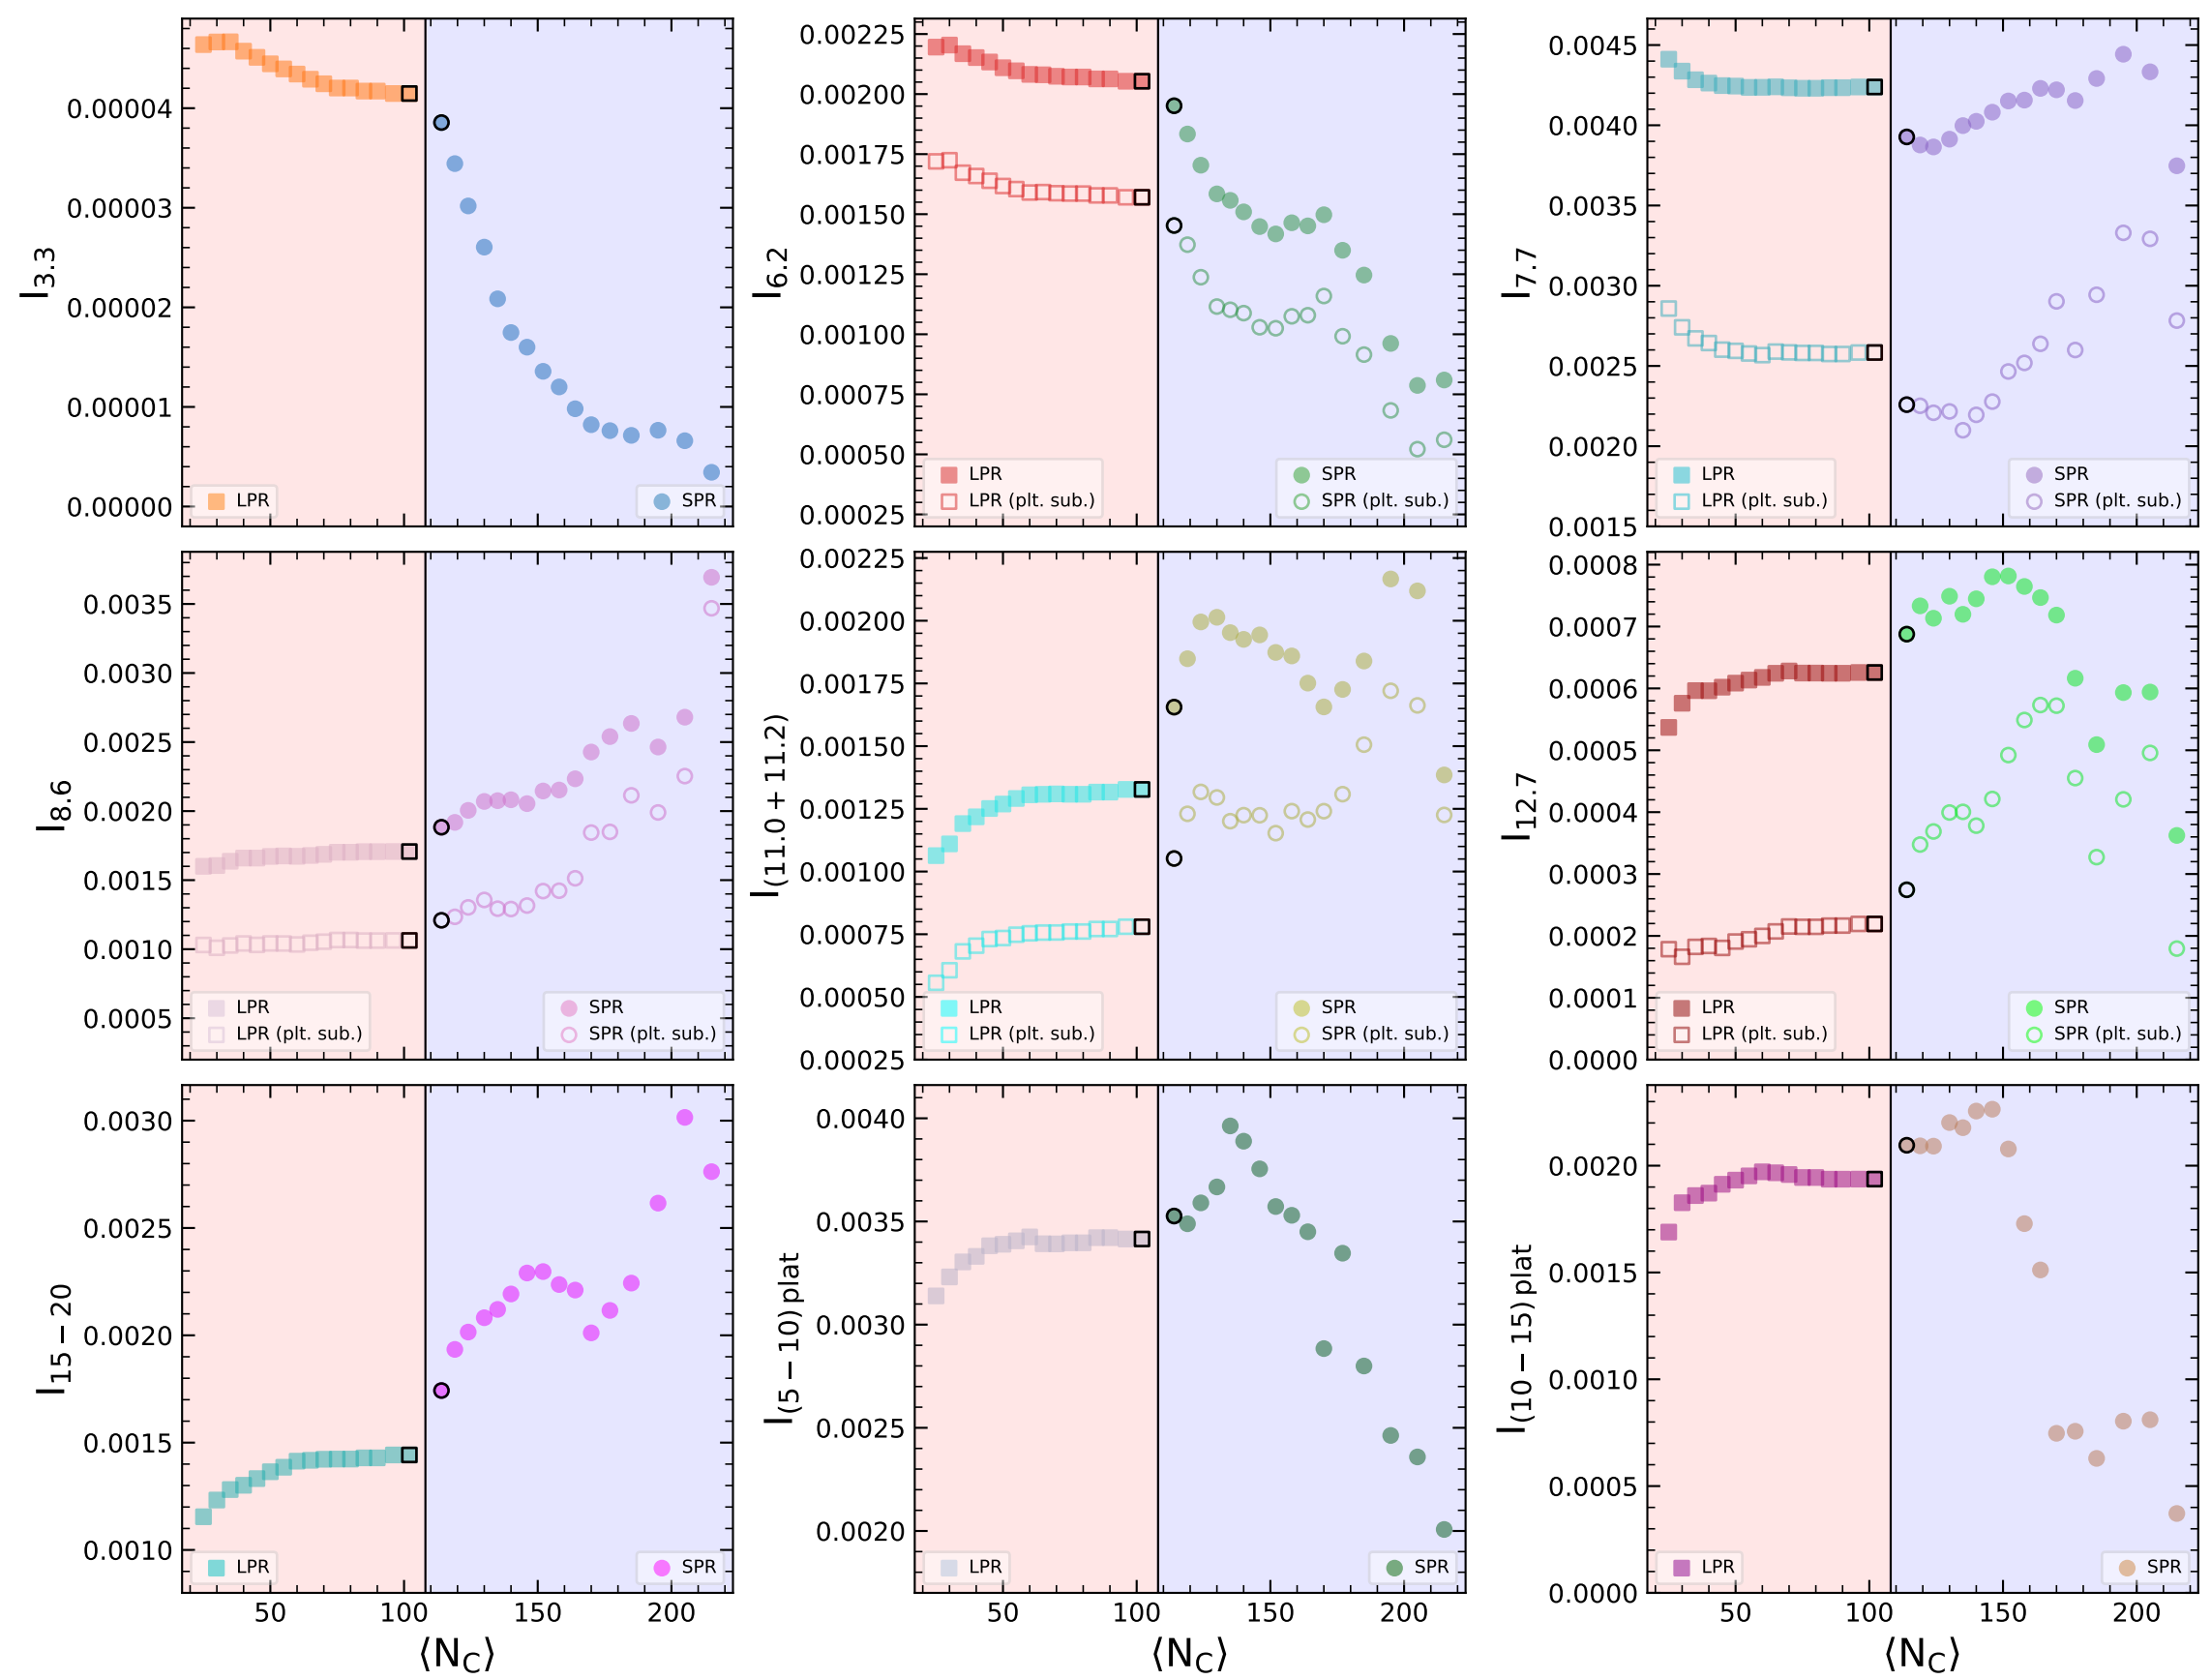

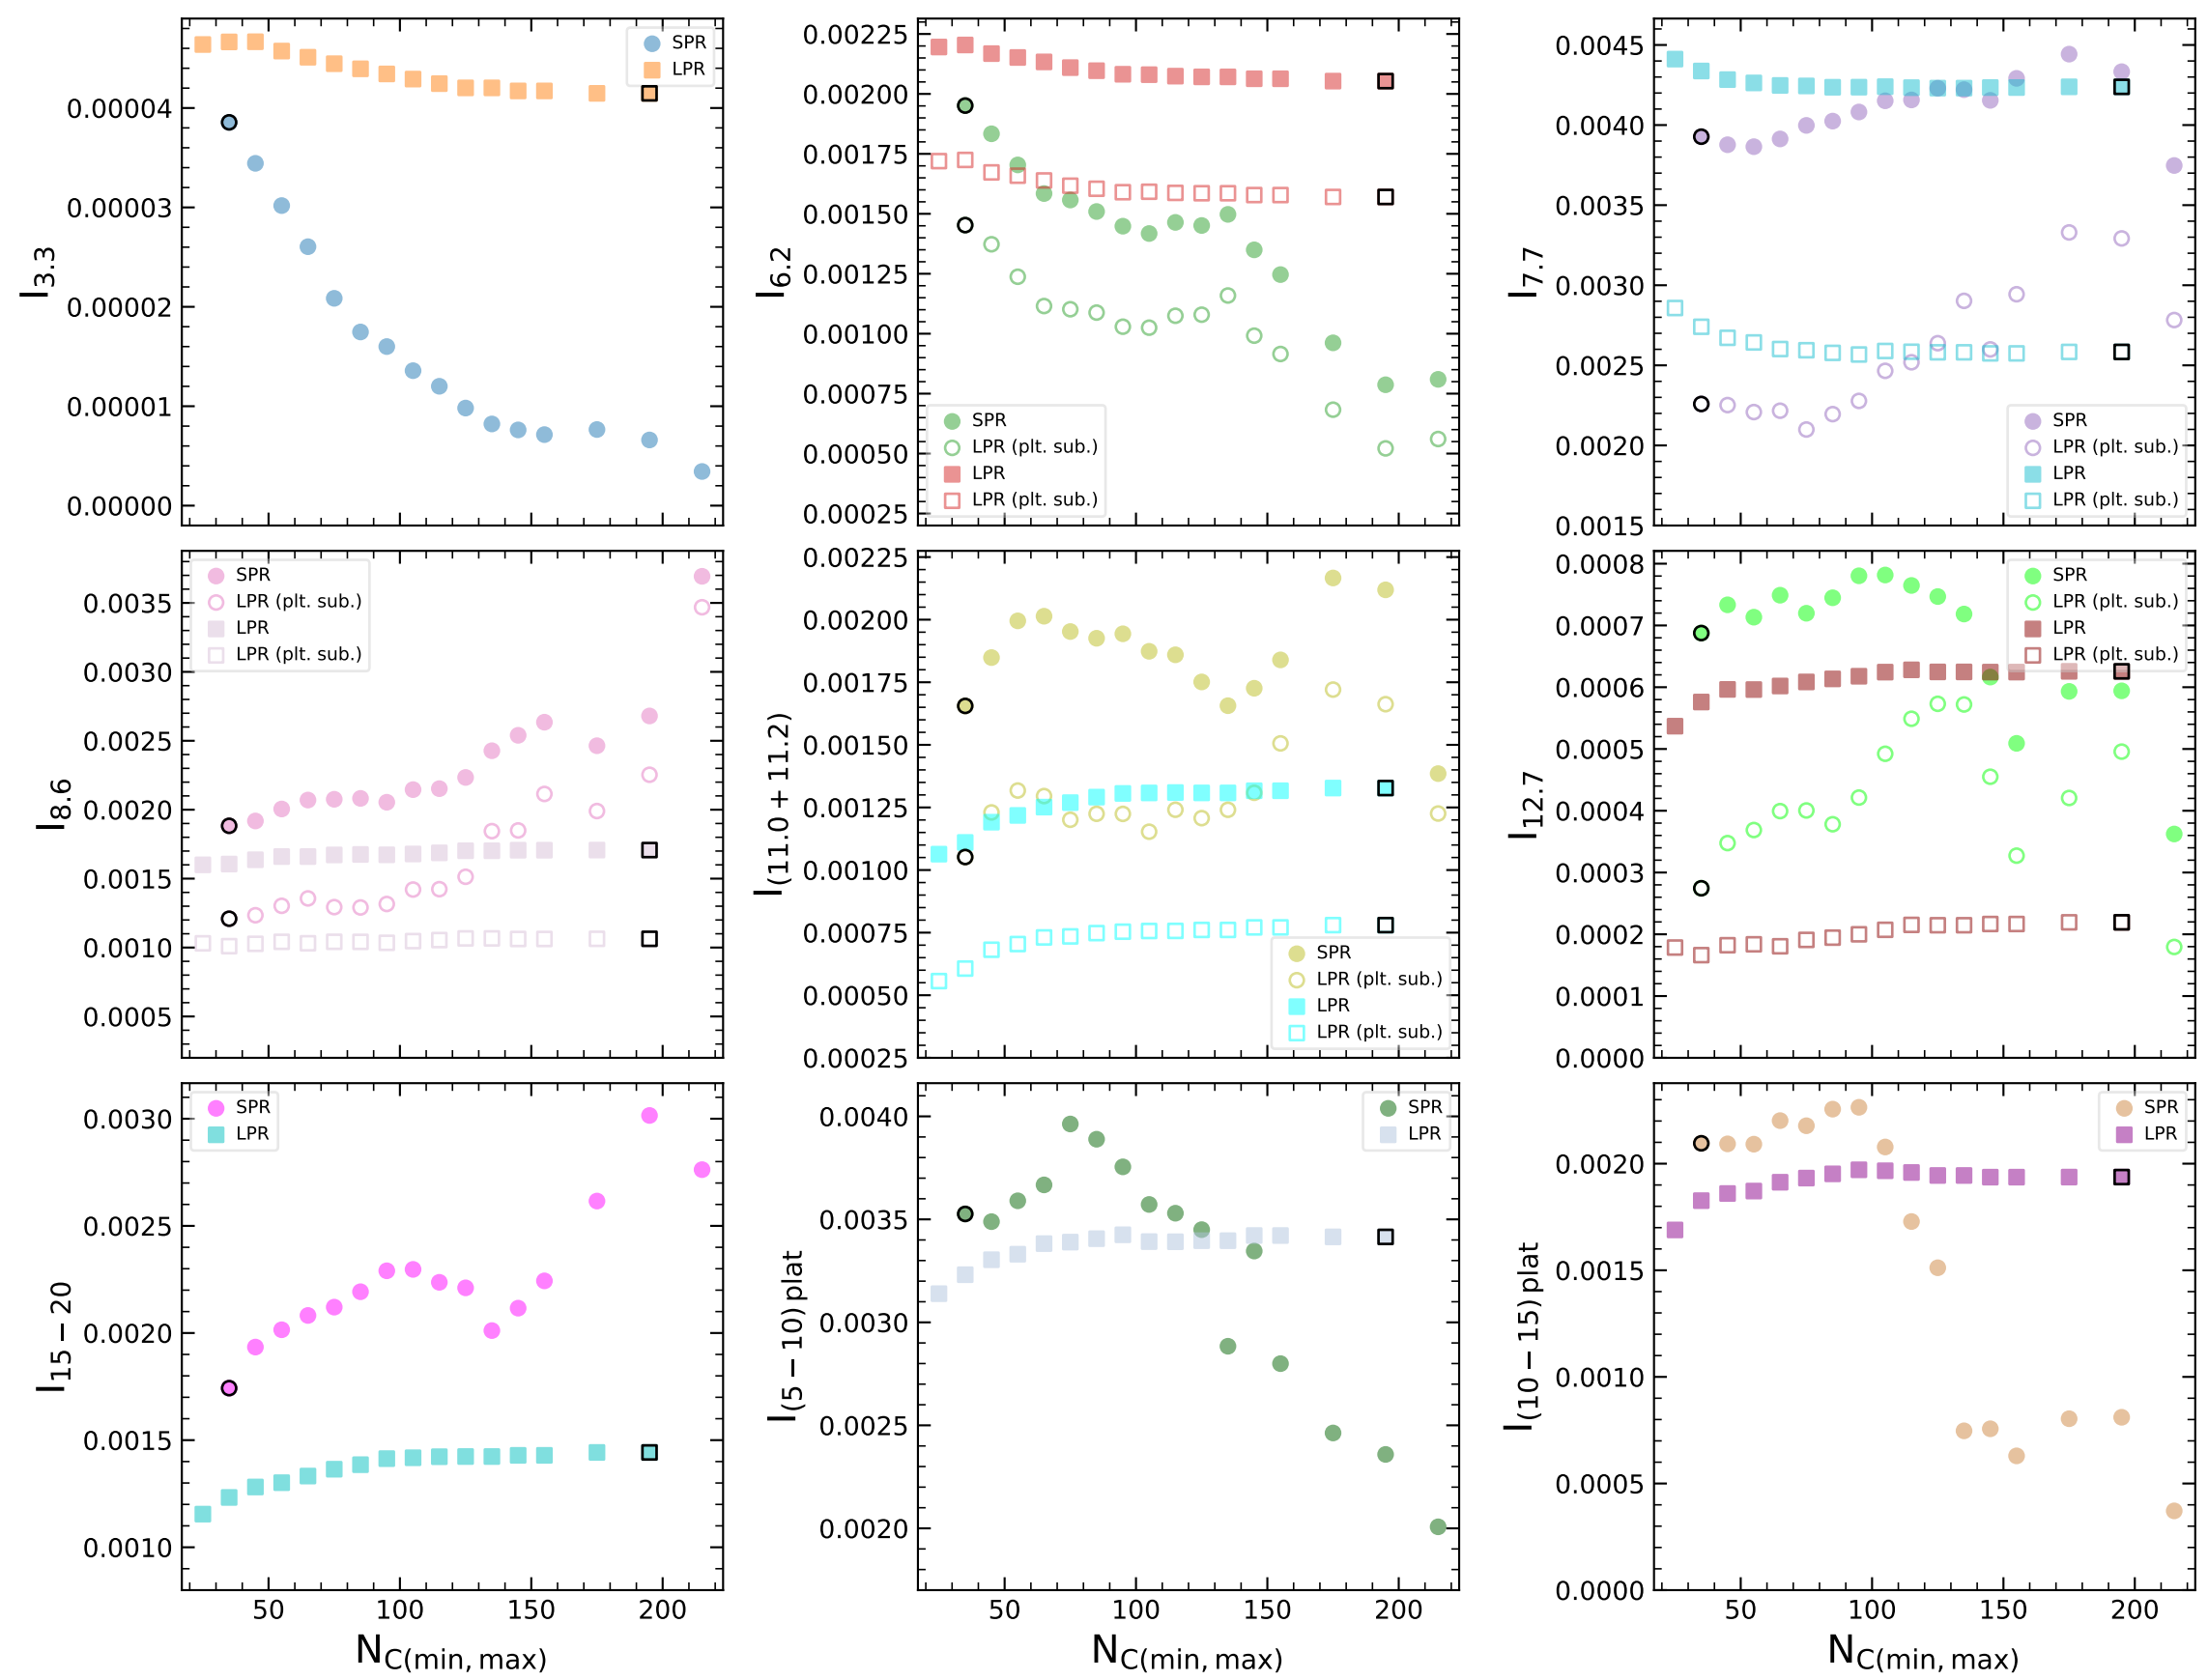

$$3.3/(11.0+11.2)$$

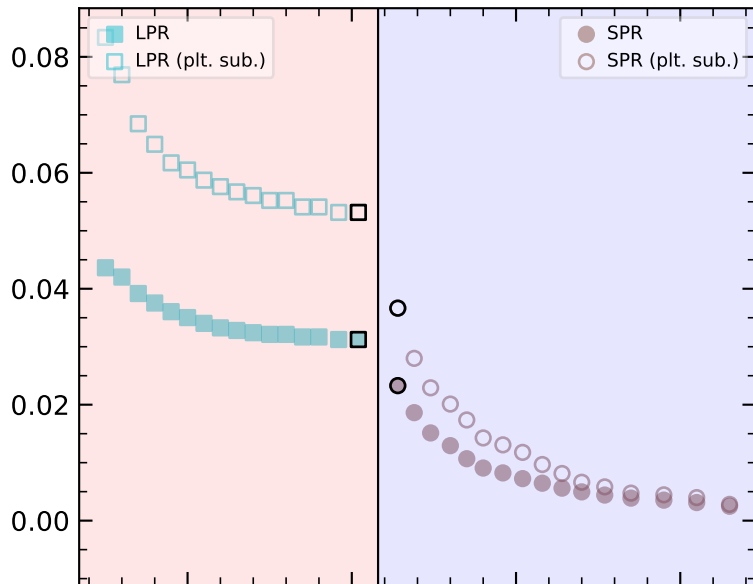

$$7.7/(11.0+11.2)$$

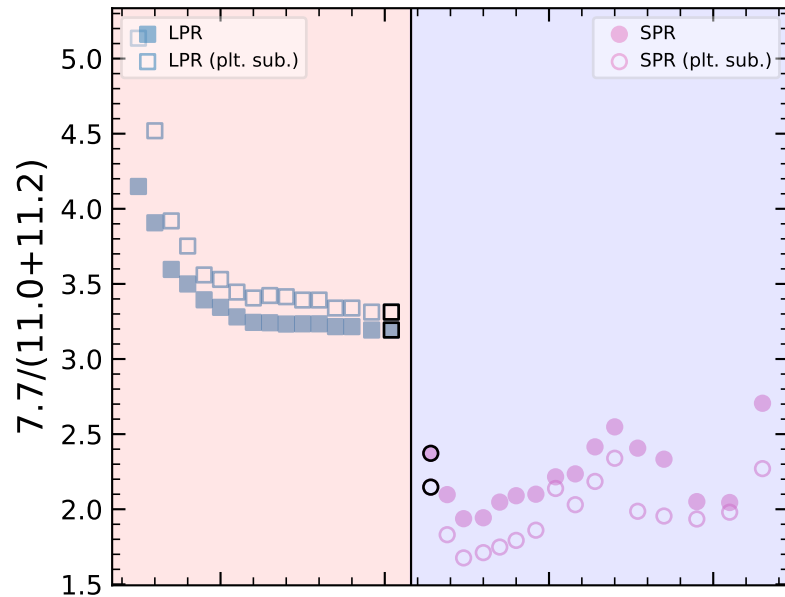

$$6.2/(11.0+11.2)$$

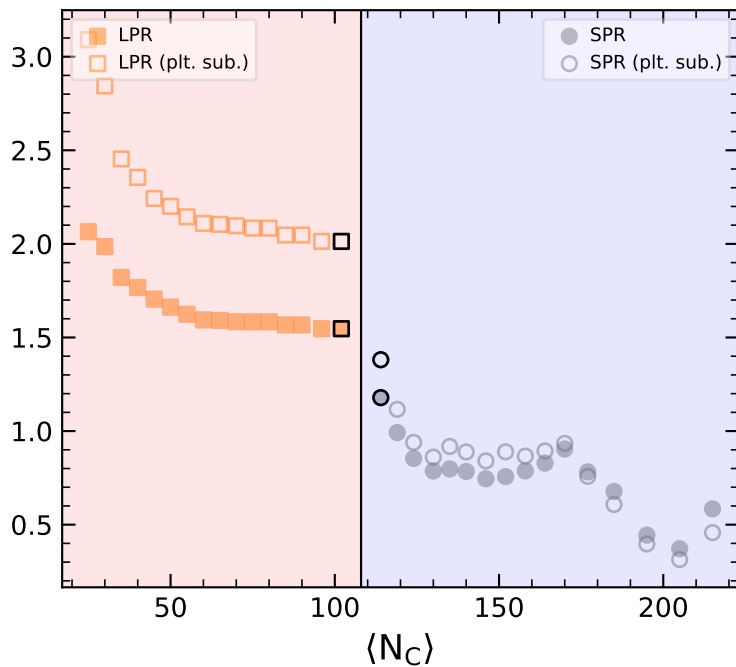

$$8.6/(11.0+11.2)$$

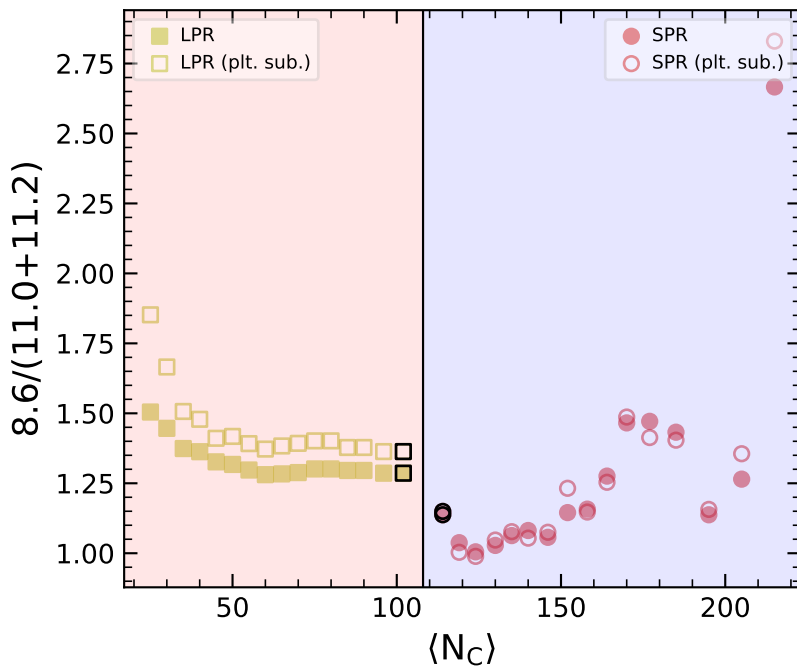

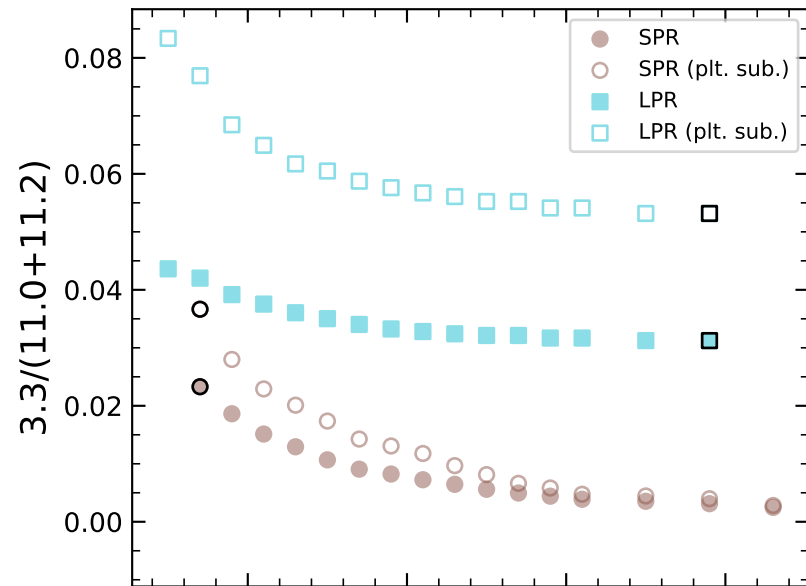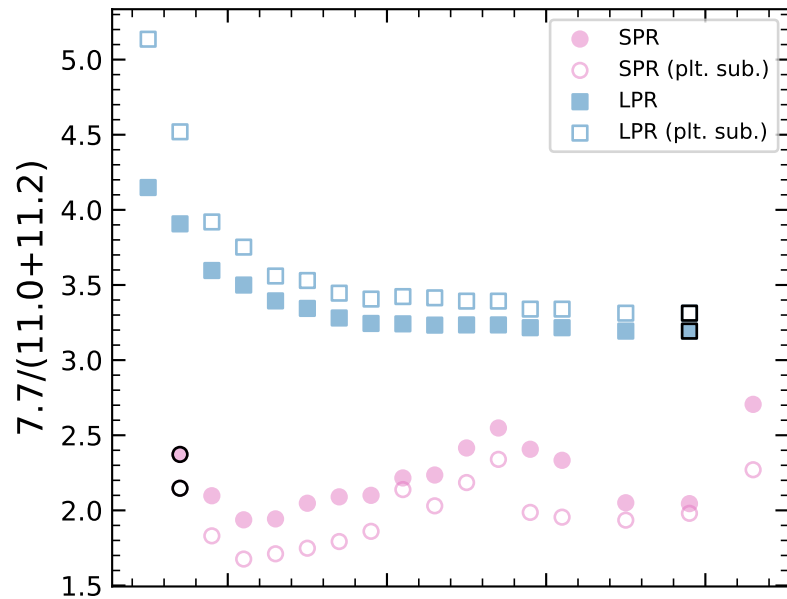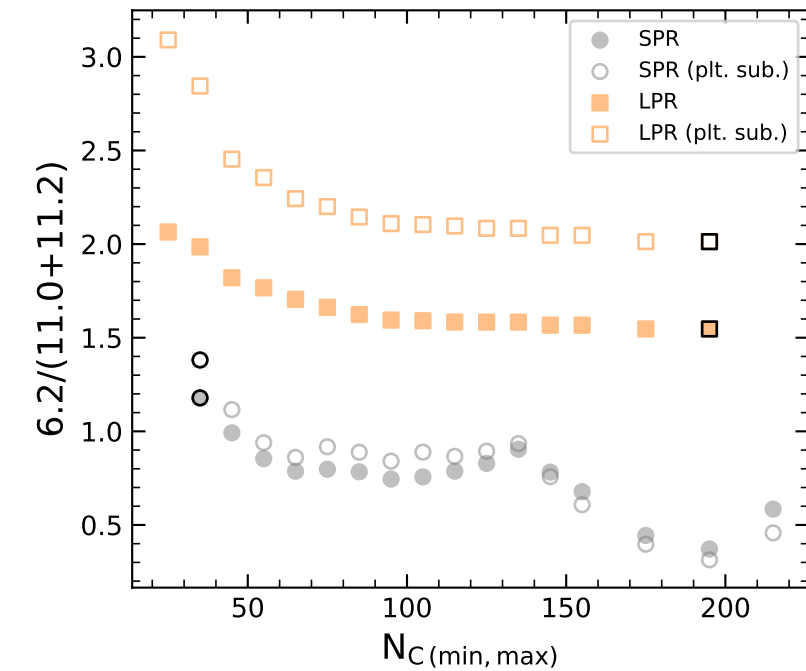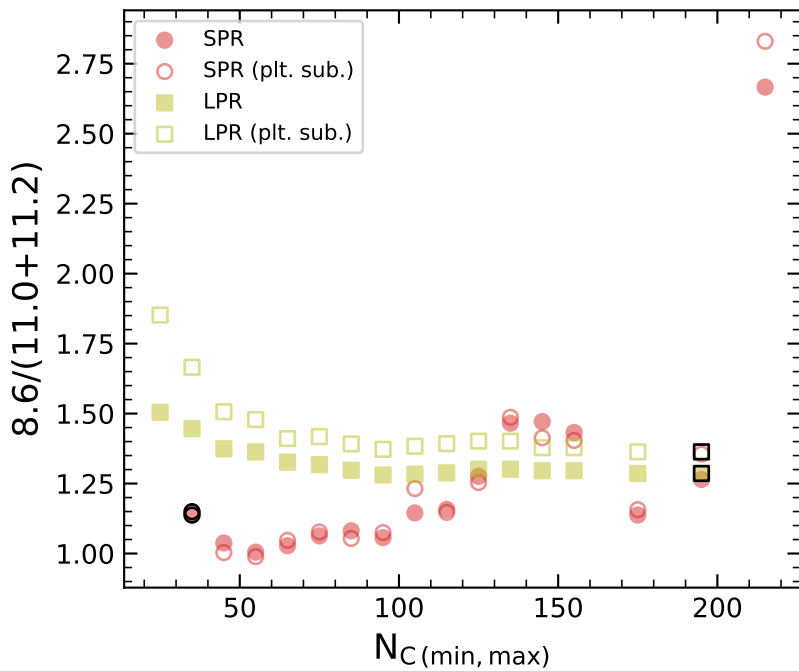

Supplement: Supplementary file 1 [file Cation_plots_v02.pdf]
