# Supplementary material for: Spectral variations among different scenarios of PAH processing or formation
Source: arXiv:2302.03678 source file (2023-02-07)

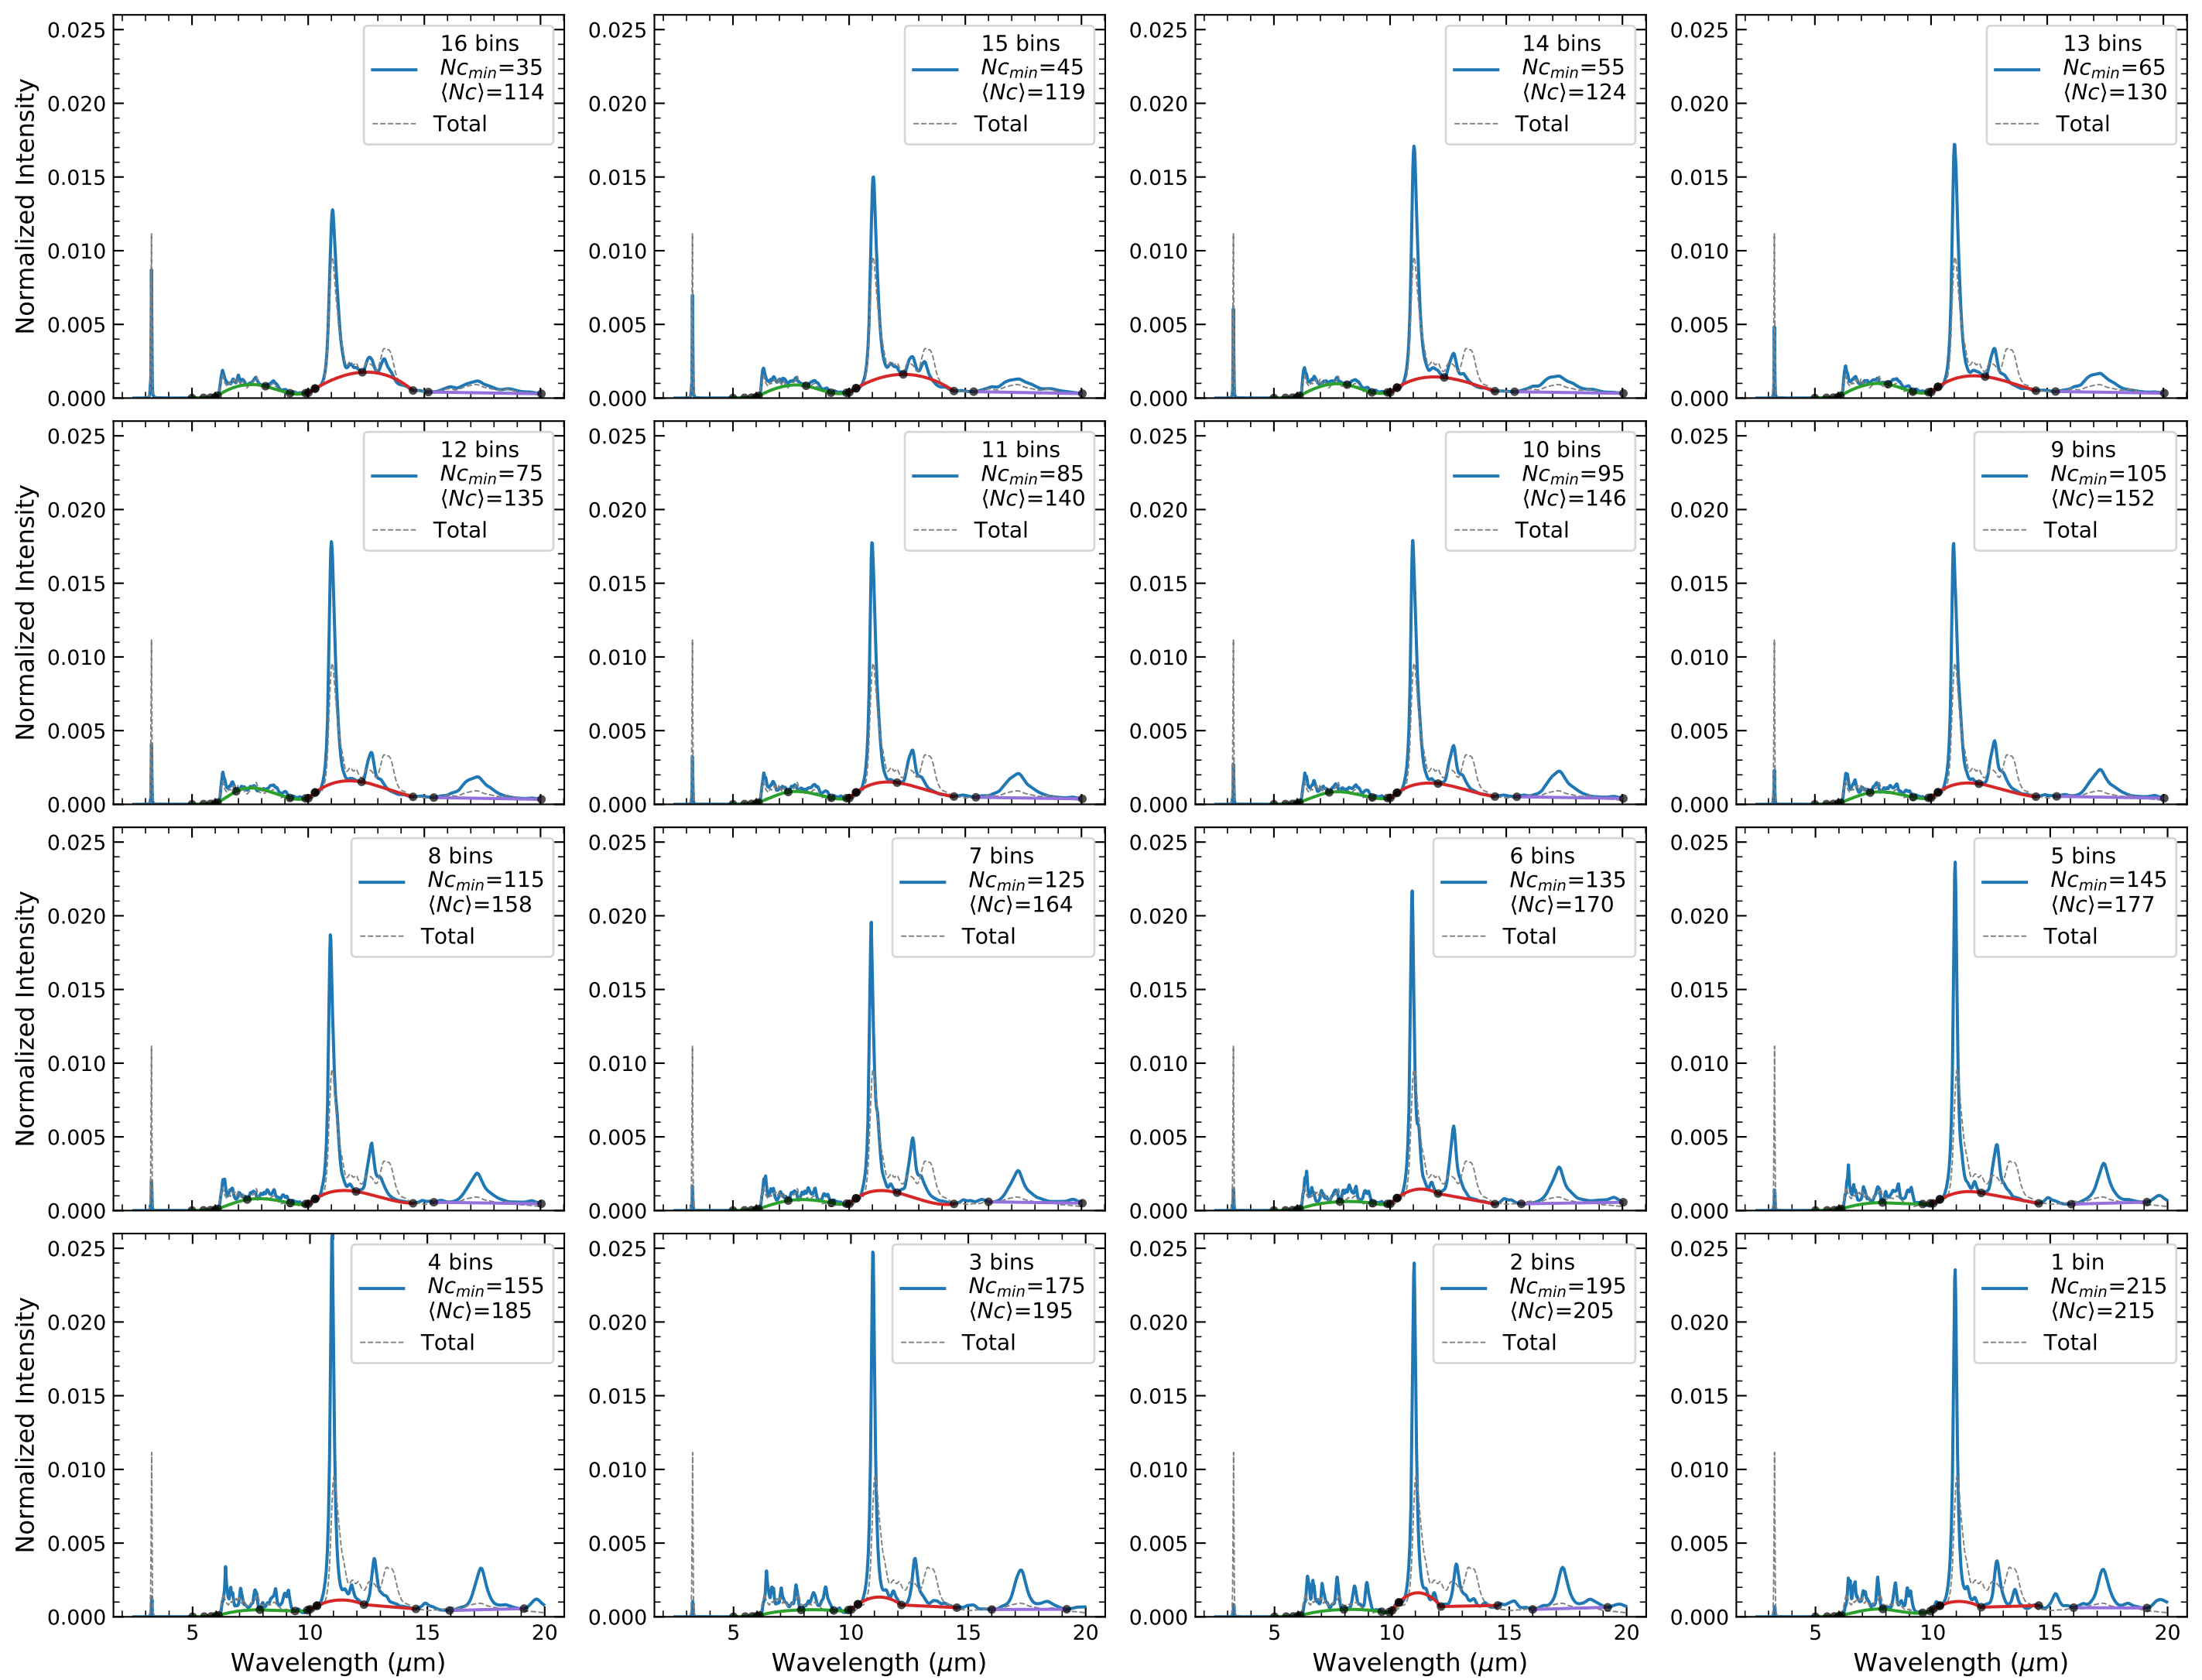

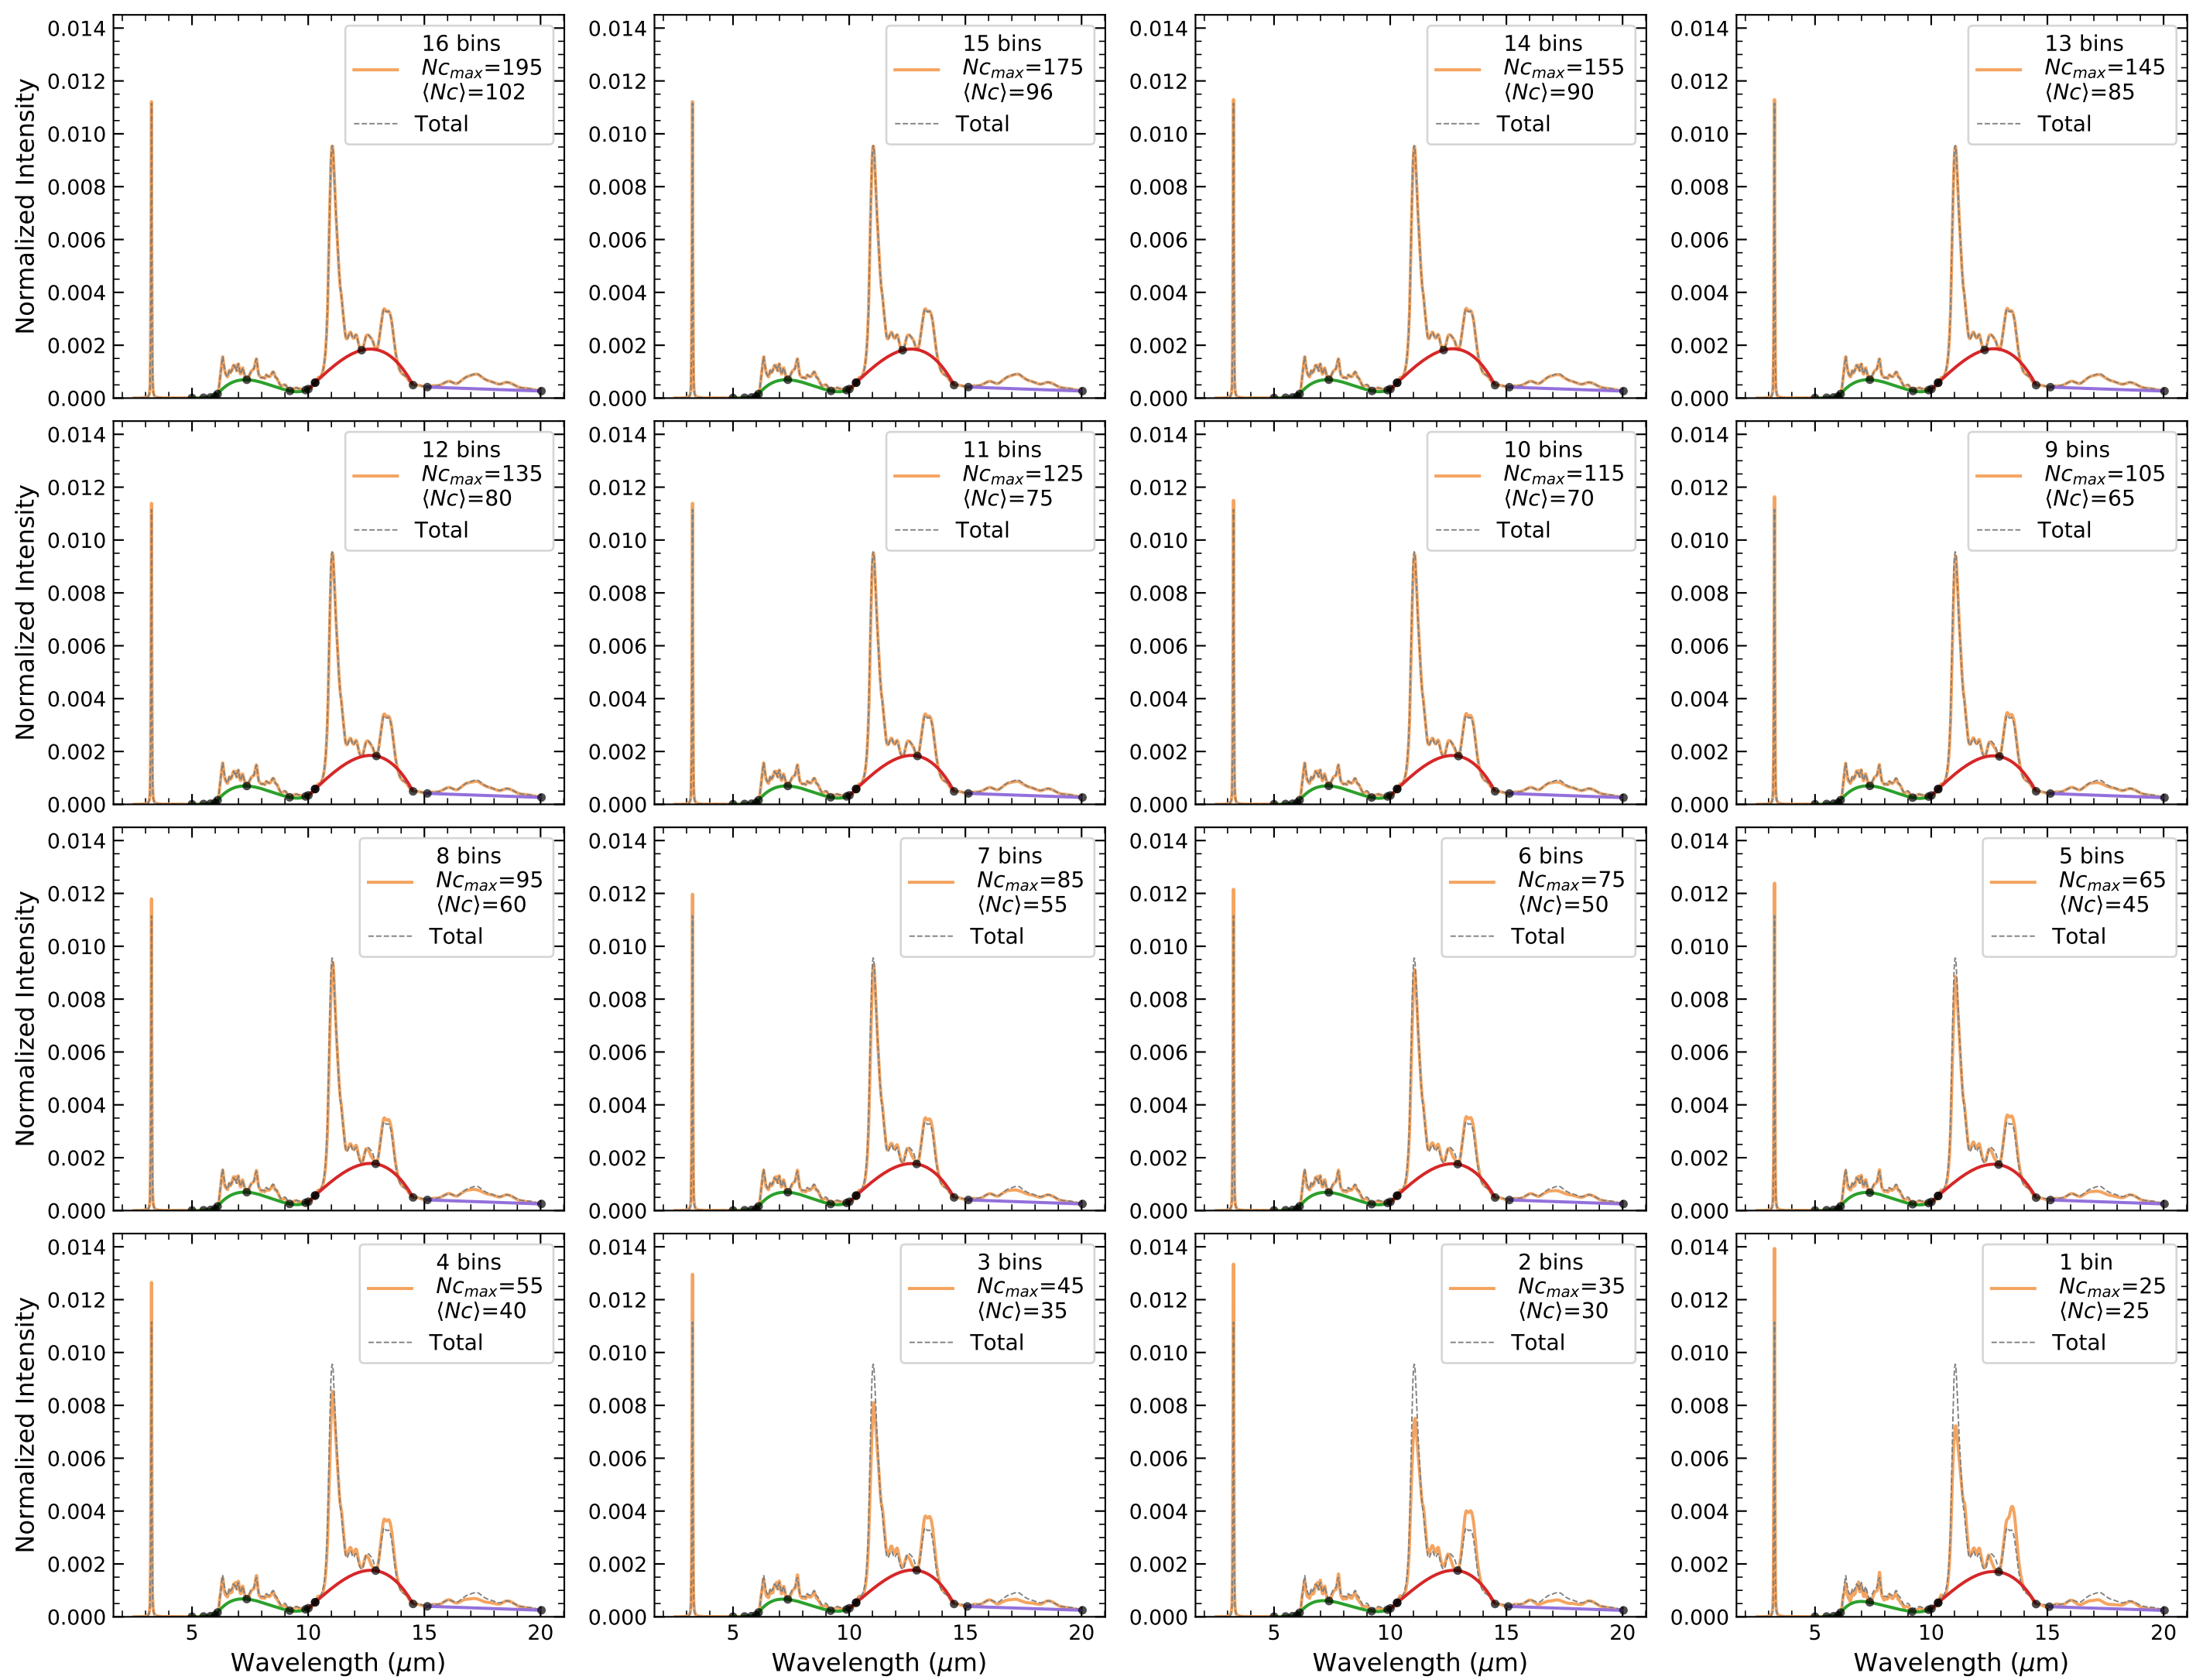

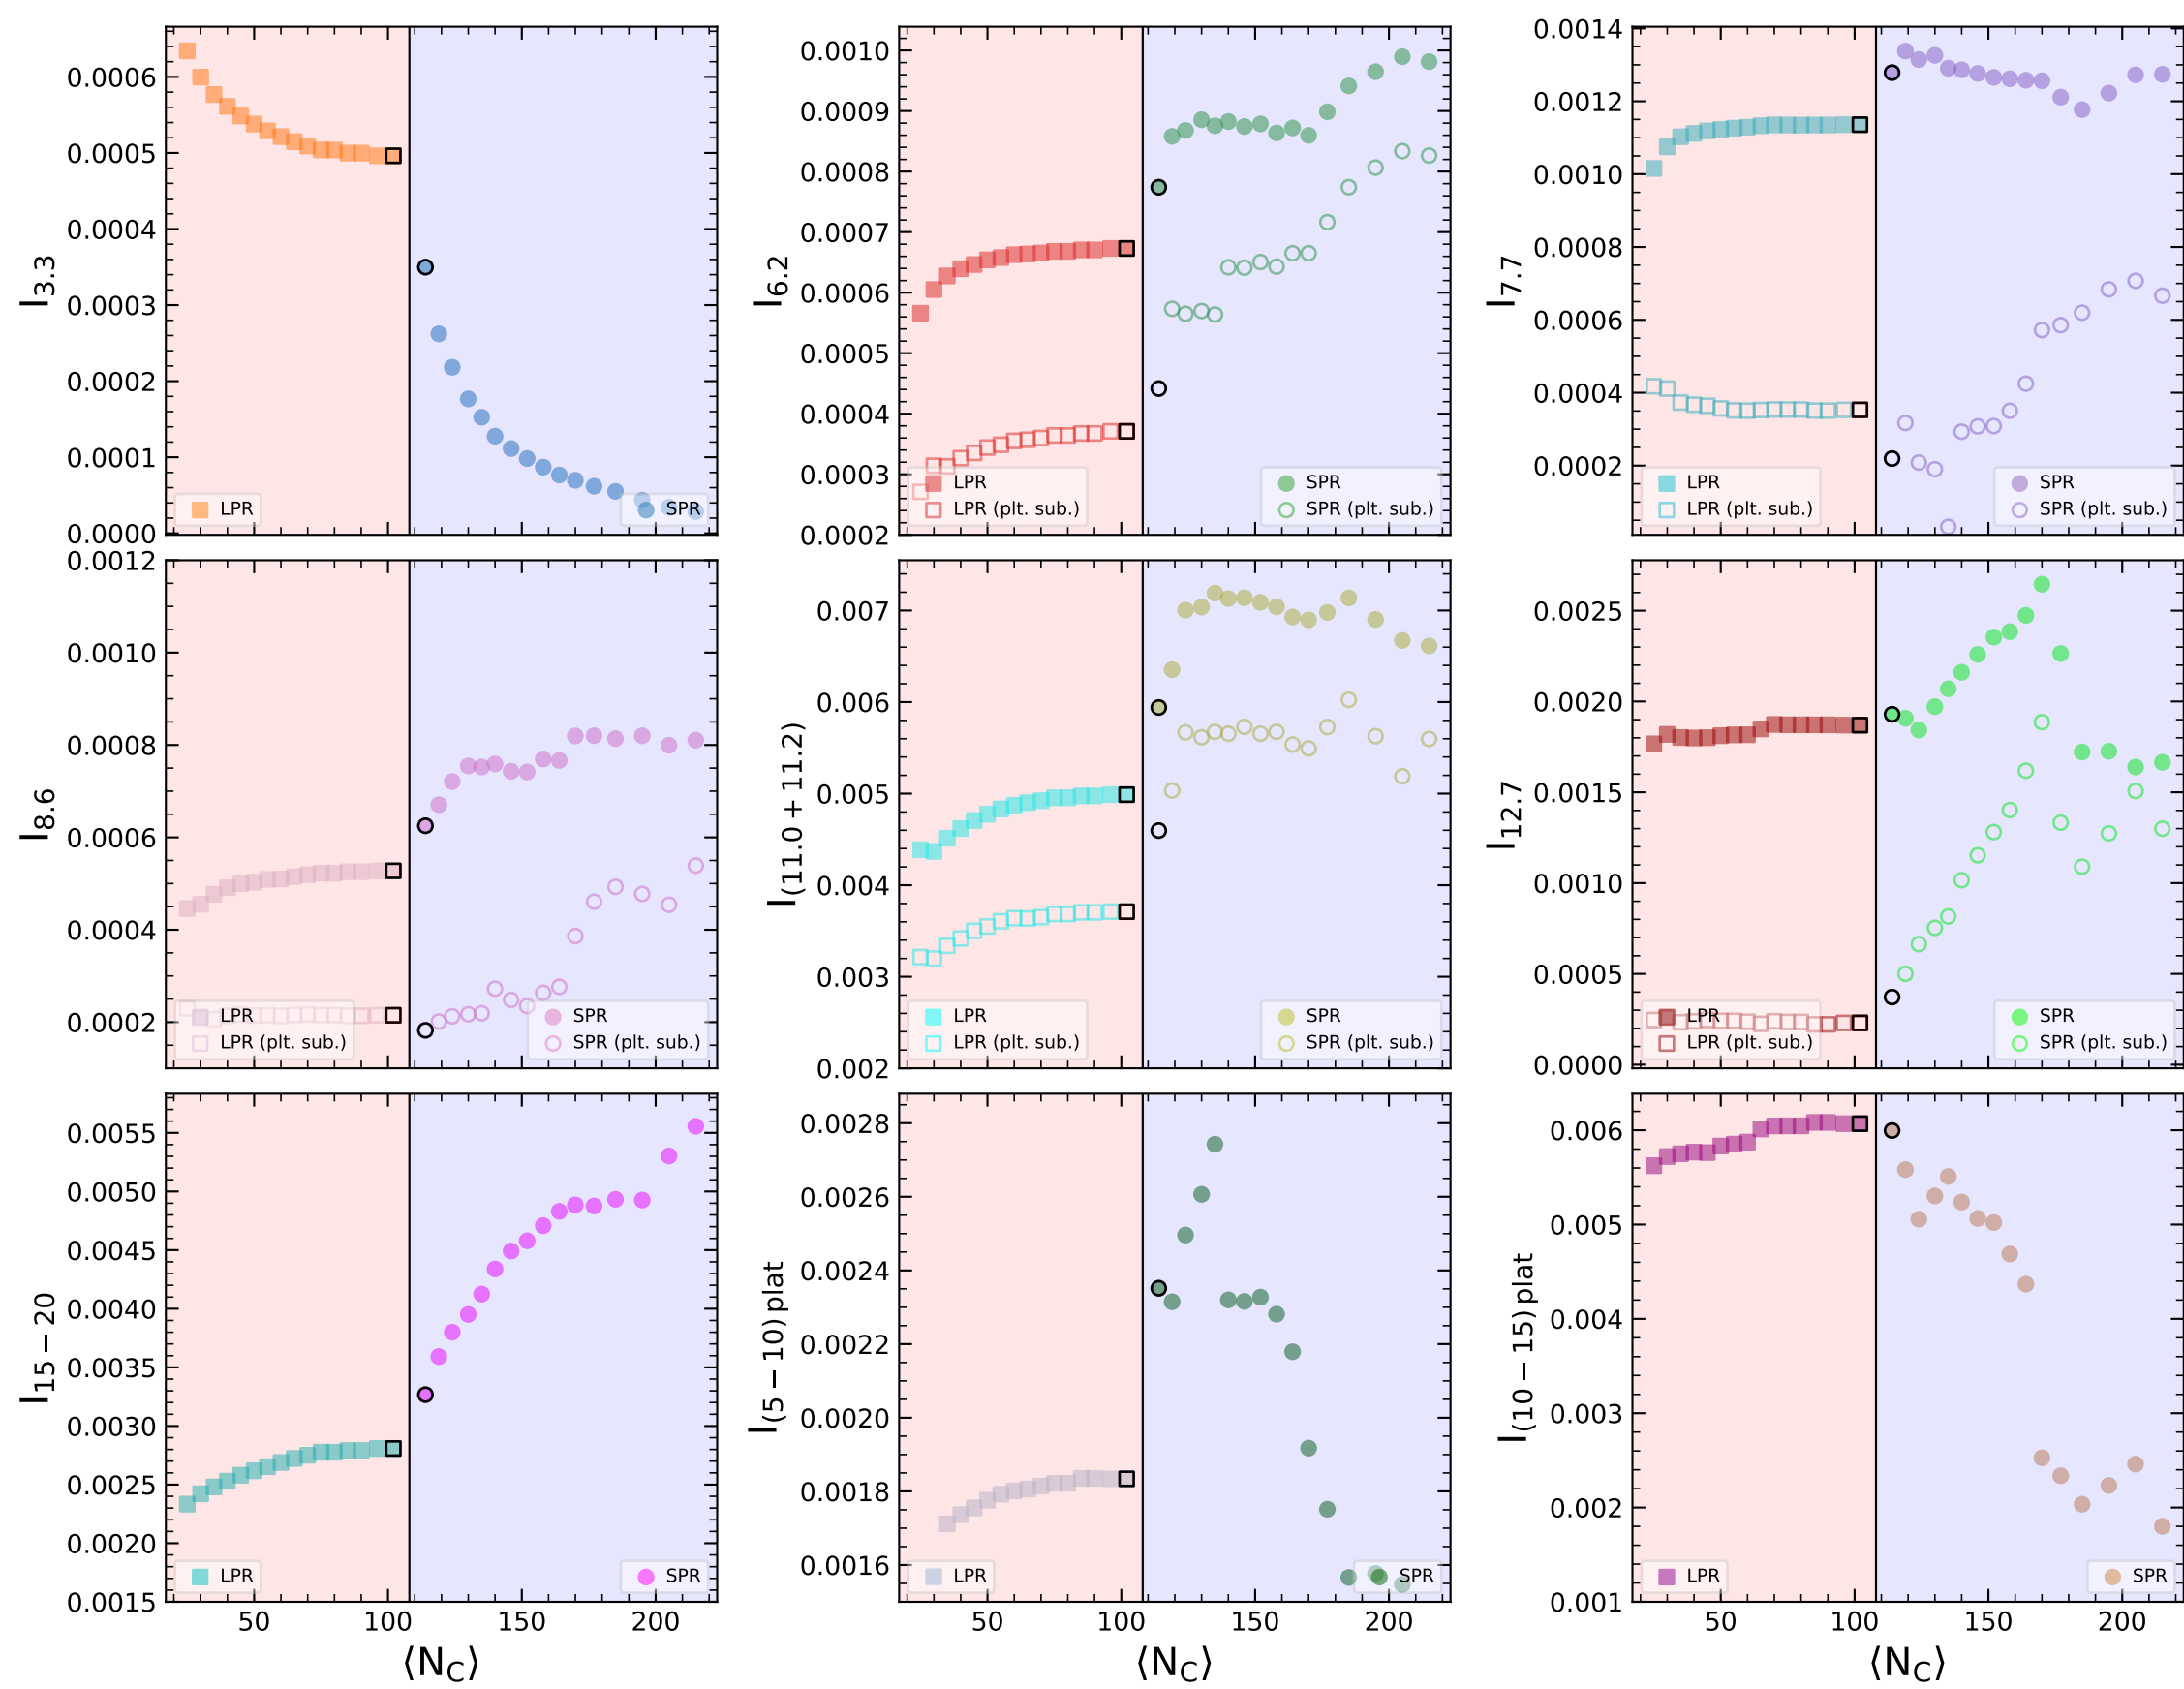

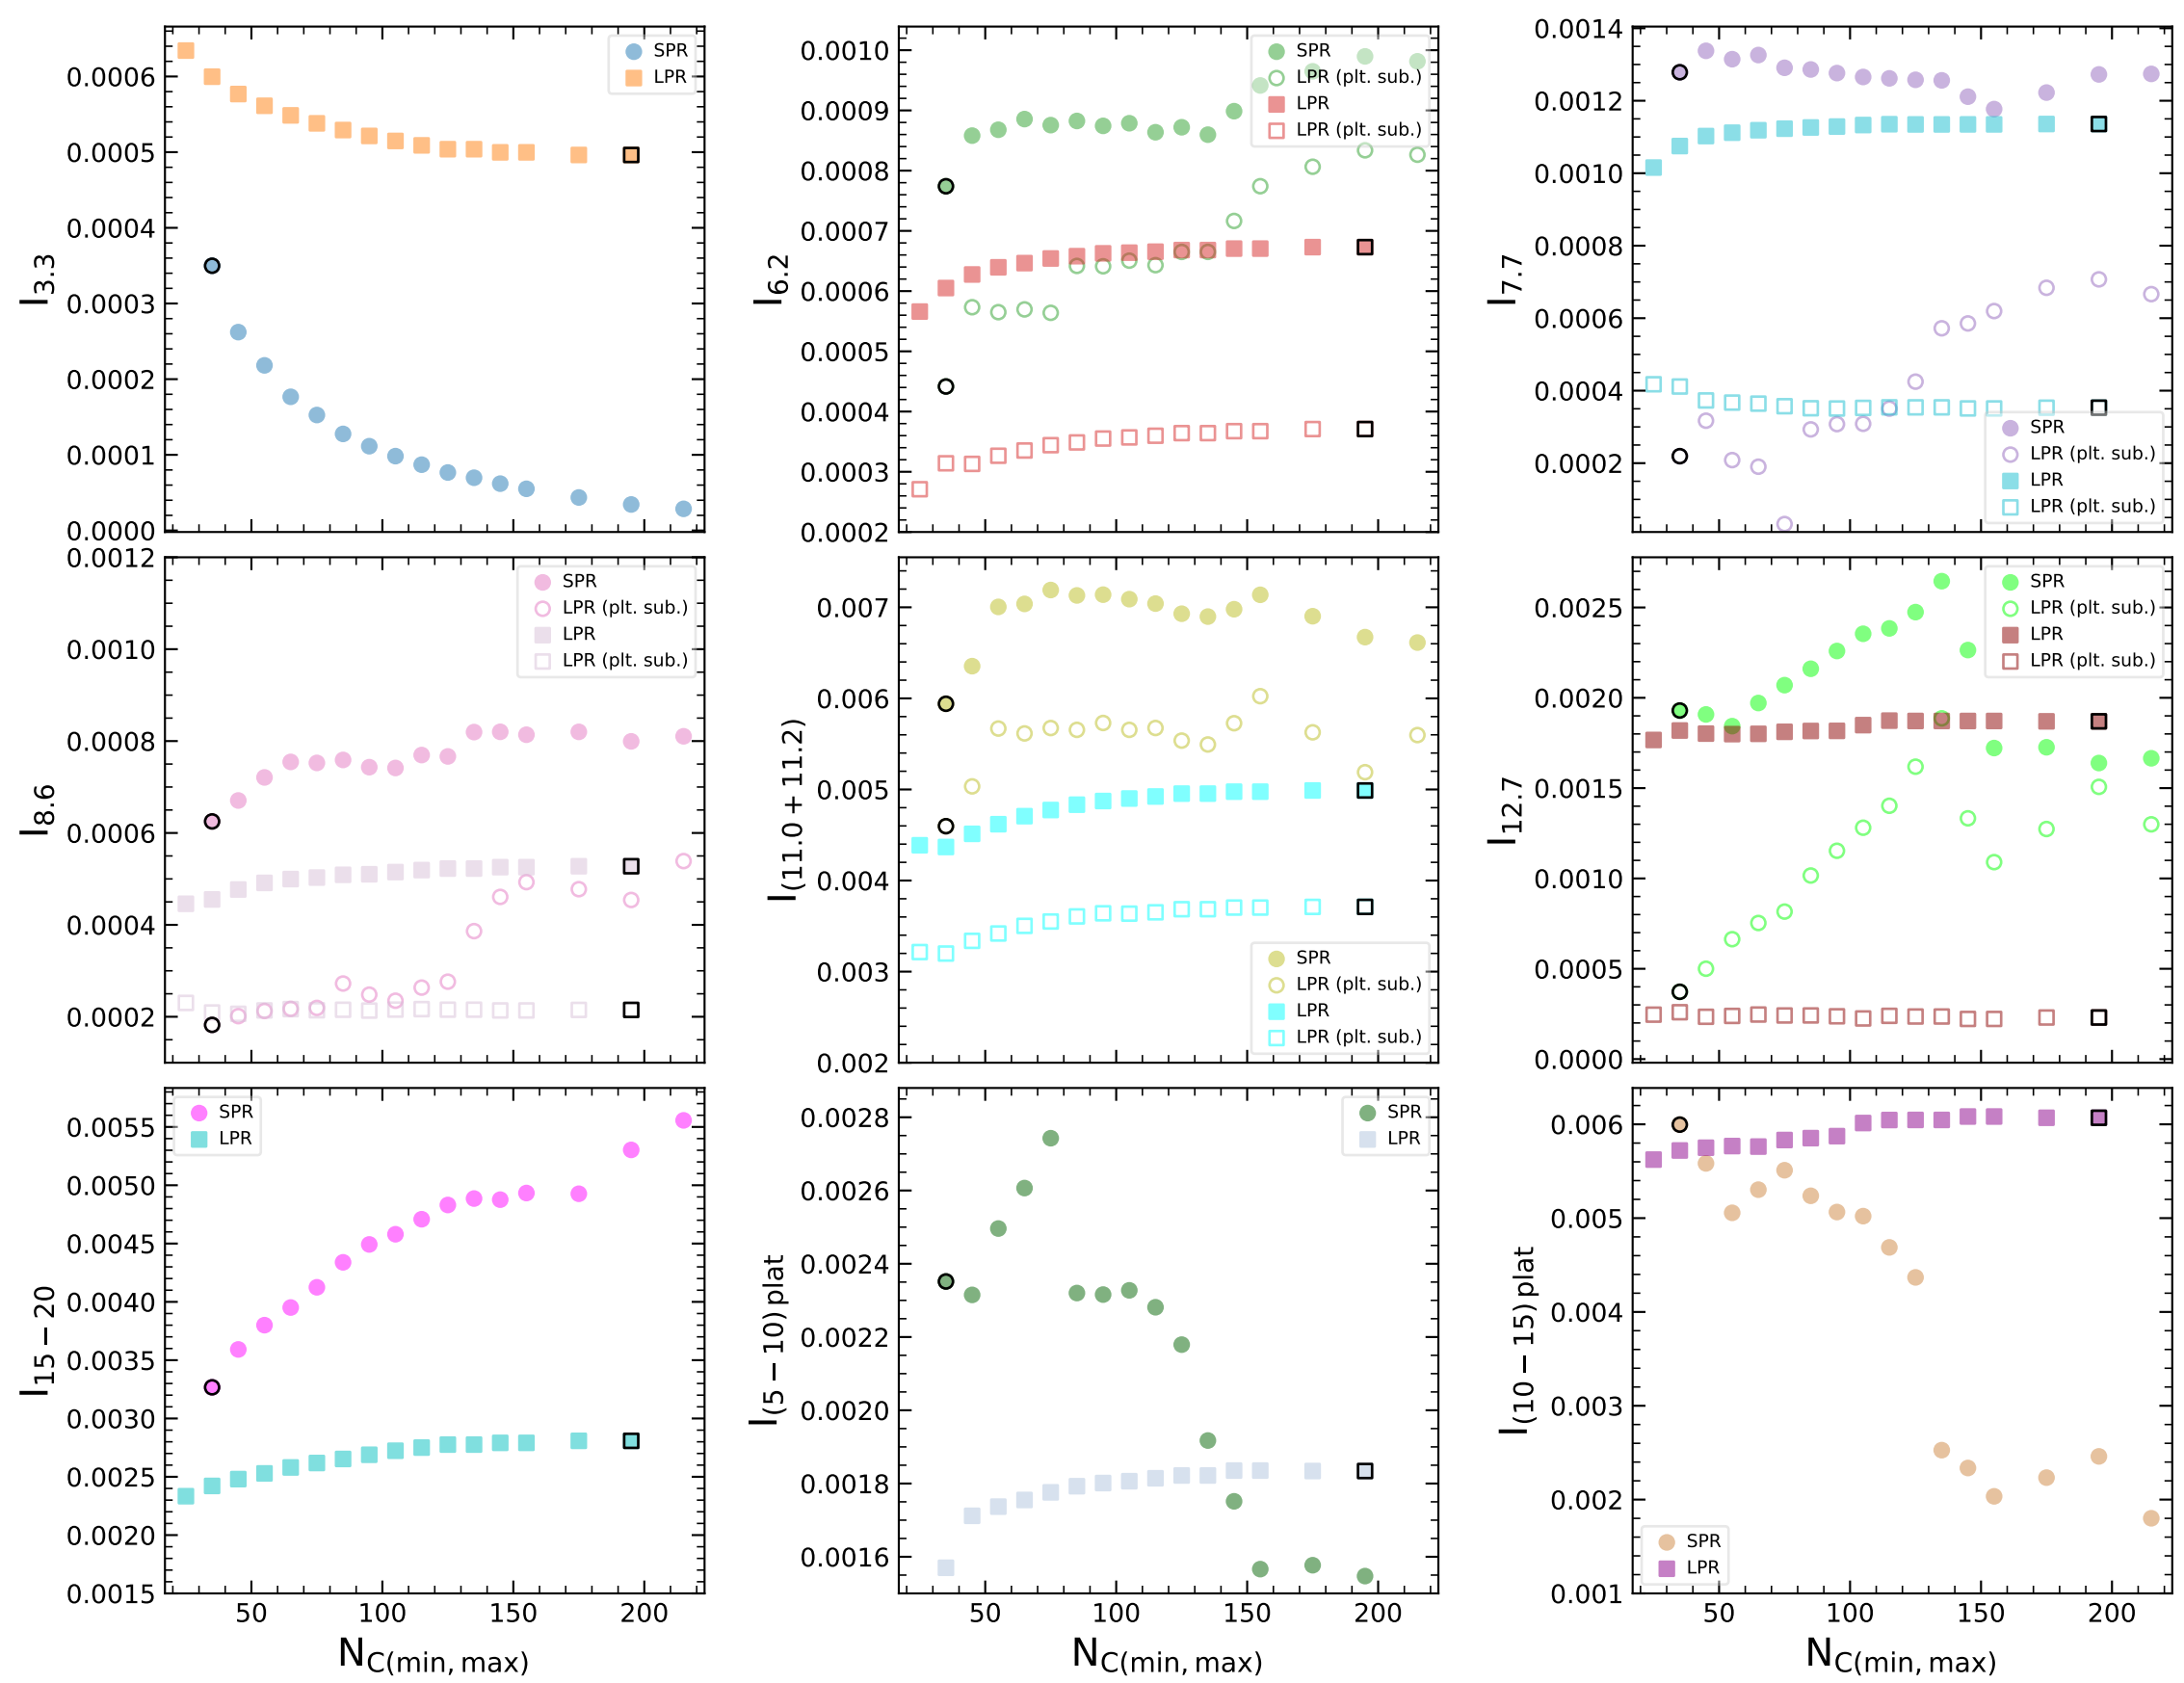

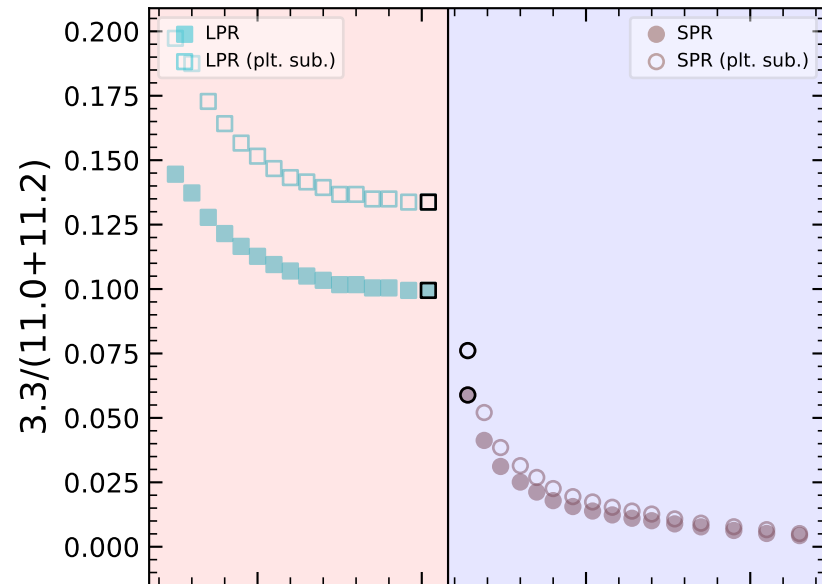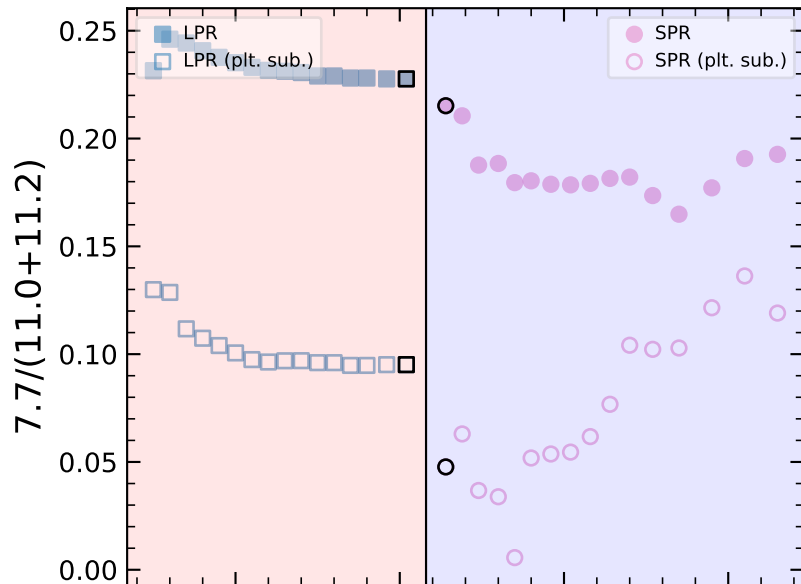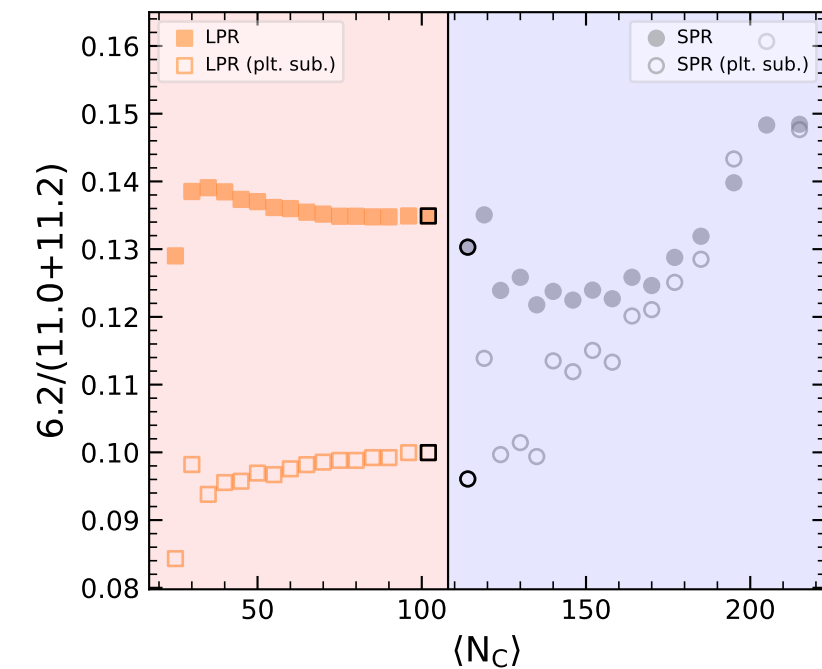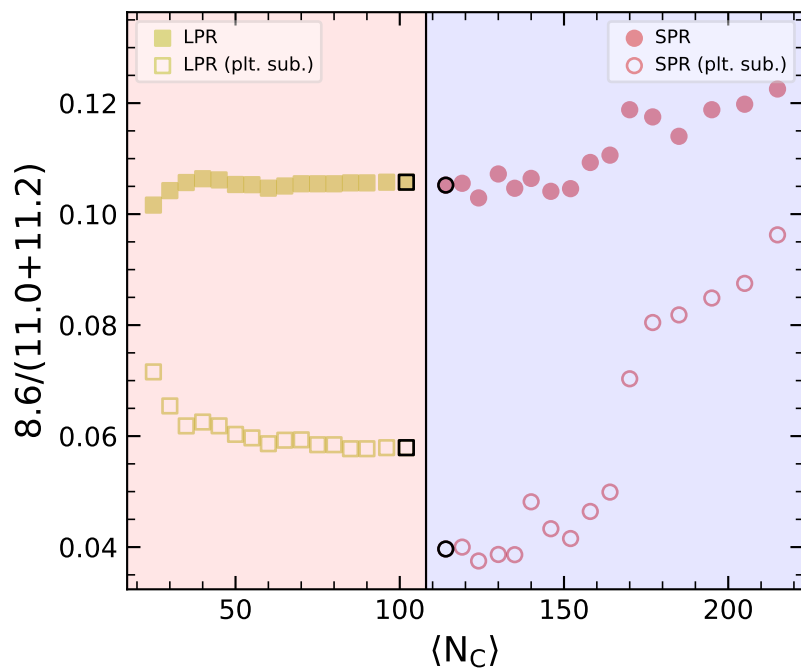

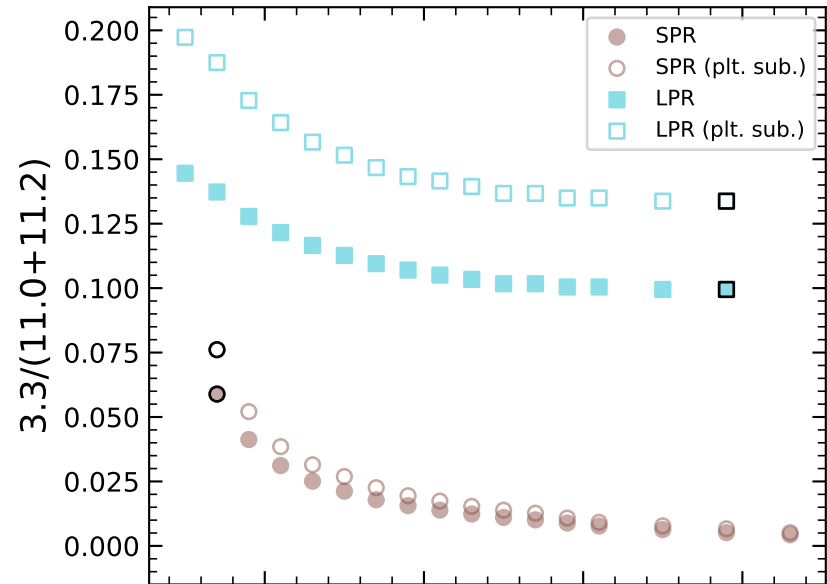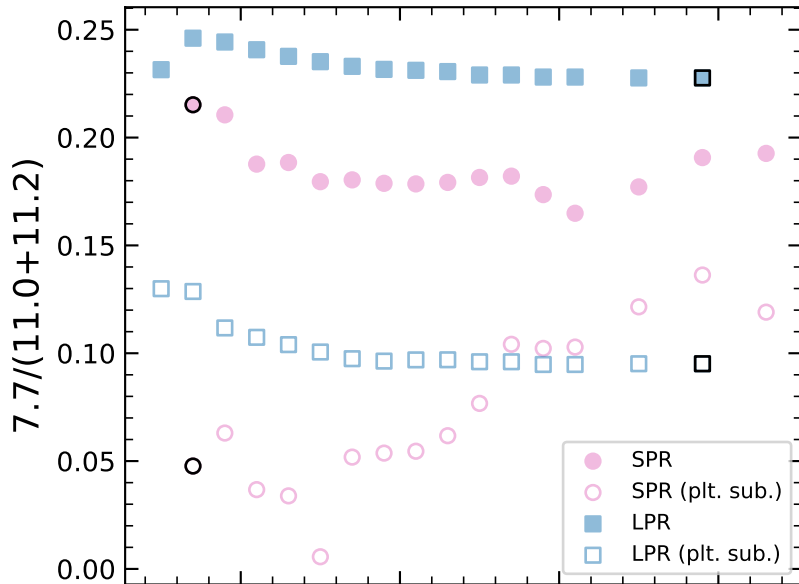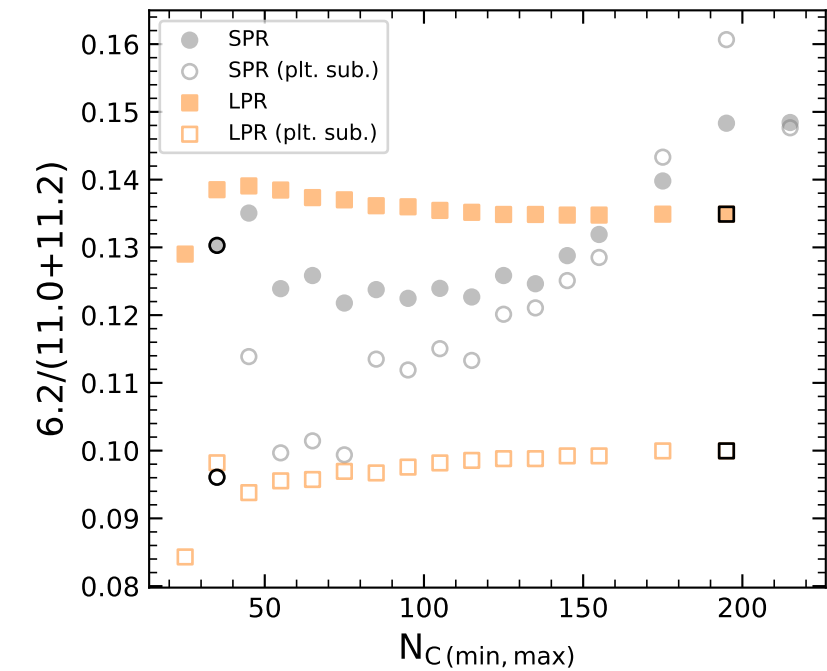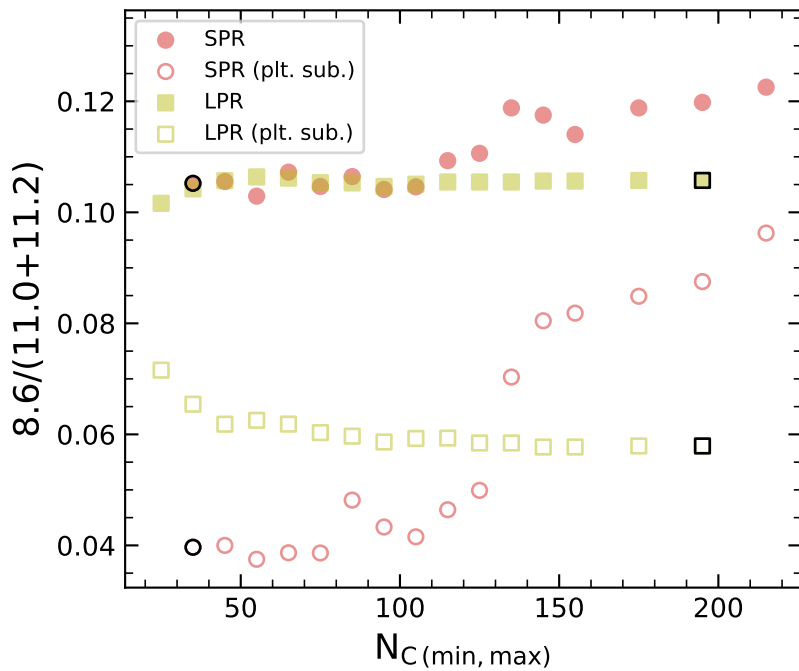

Supplement: Supplementary file 4 [file Neutral_plots_v02.pdf]
